# Supplementary material for: The Triply-Randomized Negative Binomial Beta for Robust Regression and Conjugate Models of Bounded Support Data
Source: arXiv:2606.11624 source file (2026-06-10)
Supplement: Supplementary file 1 [file appendix.tex]

\makeatletter
\let\origequation\equation
\let\origendequation\endequation
\expandafter\let\expandafter\origequationstar\csname equation*\endcsname
\expandafter\let\expandafter\origendequationstar\csname endequation*\endcsname
\let\origtheHproposition\theHproposition
\let\origtheHcor\theHcor
\let\origtheHtheorem\theHtheorem
\makeatother
\makeatletter
\newcommand{\restatealiasOn}{%
  \let\bodylabel\@gobble
  \let\equation\origequationstar
  \let\endequation\origendequationstar
  \renewcommand{\theHproposition}{restate.\arabic{proposition}}%
  \renewcommand{\theHcor}{restate.\arabic{cor}}%
  \renewcommand{\theHtheorem}{restate.\arabic{theorem}}%
}
\newcommand{\restatealiasOff}{%
  \let\bodylabel\label
  \let\equation\origequation
  \let\endequation\origendequation
  \let\theHproposition\origtheHproposition
  \let\theHcor\origtheHcor
  \let\theHtheorem\origtheHtheorem
}
\makeatother

%%%%%%%%%%%%%%%%%%%%%%%%%%%%%%%%%%%%%%%%%%%%%%%%%%%%%%%%%%%
% Appendix A: Proofs for the TNBbeta Distribution
%%%%%%%%%%%%%%%%%%%%%%%%%%%%%%%%%%%%%%%%%%%%%%%%%%%%%%%%%%%

\section{Proofs for~\Cref{sec:dist}}\label{app:proof1}

\restatealiasOn
\noindent\textbf{\Cref{theorem:tnbebta}} (\thmMedianTwoTitle). {\itshape\propMedianTwoBody}
\restatealiasOff
\begin{proof}
\textit{Part (1).} We first show that if $X \sim \mathrm{LNbeta}\big(\varepsilon,\,\varepsilon,\,\tfrac{1-p}{p}\big)$ then $\mathrm{median}(X) \teq p$. Define the map $x \teq g(y)$ as follows
\begin{equation*}
    x = \frac{y(1-p)}{y(1-p)+(1-y)p}
\end{equation*}
We show that this map transforms Libby-Novick beta density into the symmetric beta density $\textrm{beta}(\varepsilon,\,\varepsilon)$. Let $D = y(1-p)+(1-y)p$. Then the Jacobian is
\begin{equation*}
    \frac{dx}{dy} = \frac{(1-p)D - y(1-p)(1-2p)}{D^2} = \frac{p(1-p)}{D^2}
\end{equation*}
which is positive, so the map is strictly increasing. Under the map $g$, $x = \nicefrac{y(1-p)}{D}$ and $1-x = \nicefrac{(1-y)p}{D}$, so
\begin{equation*}
    x^{\varepsilon-1}(1-x)^{\varepsilon-1} = \frac{\big(y(1-p)\big)^{\varepsilon-1}\big((1-y)p\big)^{\varepsilon-1}}{D^{2(\varepsilon-1)}}
\end{equation*}
Therefore the change-of-variables formula $f_X(x)\,|dx/dy| = f_Y(y)$:
\begin{equation*}
    \underbrace{\frac{x^{\varepsilon-1}(1-x)^{\varepsilon-1}}{B(\varepsilon,\varepsilon)}}_{\text{beta}(\varepsilon,\varepsilon)} \cdot \frac{p(1-p)}{D^2}
    = \frac{y^{\varepsilon-1}(1-y)^{\varepsilon-1}}{B(\varepsilon,\varepsilon)} \cdot \frac{(1-p)^\varepsilon p^\varepsilon}{D^{2\varepsilon}}
\end{equation*}
which recovers the Libby-Novick beta density as desired. Now because $g(y)$ is strictly increasing, the median $m$ of $X$ satisfies
\begin{equation*}
    \mathbb{P}\big(X \le m\big) = \tfrac{1}{2} \iff \mathbb{P}\big(Z \le g(m)\big) = \tfrac{1}{2}
\end{equation*}
The median of $Z \sim \mathrm{beta}(\varepsilon,\varepsilon)$ is $\tfrac{1}{2}$ by symmetry, so $g(m) = \tfrac{1}{2}$. Solving:
\begin{align*}
    g(m) = &\frac{m(1-p)}{m(1-p)+(1-m)p} = \frac{1}{2} \\
    \Longleftrightarrow\quad&2m(1-p) = m(1-p)+(1-m)p \\
    \Longleftrightarrow\quad& m(1-p) = (1-m)p \\
    \Longleftrightarrow\quad& m = p
\end{align*}
Thus the median of the Libby-Novick beta under equality of its shapes is $p$.

Now, $Y \sim \textrm{TNBbeta}\big(p,\,q,\,\varepsilon\big)$ can be expressed as $Y \mid C\sim\textrm{LNbeta}\left(\varepsilon + C,\,\varepsilon + C,\,\tfrac{1-p}{p}\right)$ with $C \sim \textrm{NB}(\varepsilon,\,1-q)$ due to~\Cref{cor:K}. The marginal distribution of $Y$ is a mixture over distributions, each with median exactly $p$. Therefore, the median of $Y$ must also be $p$.

\textit{Part (2).} We evaluate the density at $y \teq p$. Note that
\begin{equation*}
    \gamma(p,\,p) = \frac{p(1\tm p)p(1\tm p)}{(2p(1\tm p))^2} = \frac{1}{4}.
\end{equation*}
Therefore $1 - 4q\gamma(p,p) = 1 - q$, and the density at $y \teq p$ is
\begin{align*}
    \TNB(p;\,p,\,q,\,\varepsilon) &= \mathrm{beta}(p; \varepsilon,\,\varepsilon) \cdot \big(4p(1-p)\big)^{-\varepsilon}\cdot \frac{(1\tm q)^\varepsilon}{(1\tm q)^{\varepsilon+1/2}}\\
    &= \mathrm{beta}(p; \varepsilon,\,\varepsilon) \cdot \big(4p(1-p)\big)^{-\varepsilon}\cdot (1\tm q)^{-1/2}.
\end{align*}
As $q \to 1$, $(1\tm q)^{-1/2} \to \infty$, so $\TNB(p;\,p,\,q,\,\varepsilon) \to \infty$.

\textit{Part (3).} Write the log-density as $\ell(y) = \ell_{\mathrm{LN}}(y;\,\varepsilon,\,p) + \varepsilon\log(1\tm q) - (\varepsilon \tp \tfrac{1}{2})\log(1 - 4q\gamma(y,p))$, where $\ell_{\mathrm{LN}}$ collects terms not involving $q$. The only term involving both $p$ and $q$ is $-(\varepsilon\tp\tfrac{1}{2})\log(1 - 4q\gamma)$. We first compute
\begin{equation*}
    \frac{\partial\gamma}{\partial p} = \frac{\partial}{\partial p}\frac{y(1\tm y)p(1\tm p)}{D^2} = \frac{y(1\tm y)(y \tm p)}{D^3}
\end{equation*}
where we have used $\frac{\partial D}{\partial p} = 1 - 2y$. Therefore
\begin{equation*}
    \frac{\partial^2 \ell}{\partial p\,\partial q} = \frac{4(\varepsilon \tp \tfrac{1}{2})\,\frac{\partial \gamma}{\partial p}}{\big(1 - 4q\gamma(y,p)\big)^2} = \frac{4(\varepsilon \tp \tfrac{1}{2})\,y(1\tm y)(y\tm p)}{D^3\big(1 - 4q\gamma(y,p)\big)^2}.
\end{equation*}
We must show $\mathcal{I}_{pq} = -\ex\!\left[\frac{\partial^2 \ell}{\partial p\,\partial q}\right] = 0$. Apply the change of variables $u \teq g(y) = \nicefrac{y(1\tm p)}{D}$ from part~(1). Setting $R = up \tp (1\tm u)(1\tm p)$, we have $D = p(1\tm p)/R$ and by direct calculation
\begin{equation*}
    y \tm p = \frac{p(1\tm p)(2u \tm 1)}{R},\qquad y(1\tm y) = \frac{u(1\tm u)p(1\tm p)}{R^2},\qquad \gamma(y,p) = u(1\tm u).
\end{equation*}
Substituting, the integrand simplifies to
\begin{equation*}
    \frac{y(1\tm y)(y\tm p)}{D^3(1 - 4q\gamma)^2}\,\mathrm{TNBbeta}(y;\,p,\,q,\,\varepsilon)\,dy = \frac{(1\tm q)^\varepsilon}{p(1\tm p)\,B(\varepsilon,\varepsilon)}\cdot\frac{u^\varepsilon(1\tm u)^\varepsilon(2u\tm 1)}{(1 - 4qu(1\tm u))^{\varepsilon+5/2}}\,du.
\end{equation*}
where again we have used the Jacobian $\frac{du}{dy} = \nicefrac{p(1-p)}{D^2}$. Since $u^\varepsilon(1\tm u)^\varepsilon$ and $(1 - 4qu(1\tm u))^{\varepsilon+5/2}$ are symmetric about $u \teq \tfrac{1}{2}$ while $(2u \tm 1)$ is antisymmetric, the integrand is antisymmetric about $u \teq \tfrac{1}{2}$. Therefore the integral over $[0,1]$ vanishes, giving $\mathcal{I}_{pq} = 0$.
\end{proof}

\restatealiasOn
\noindent\textbf{\Cref{prop:phi}} (\propPhiTitle). {\itshape\propPhiBody}
\restatealiasOff
\begin{proof}
Write $f(y) \defeq TNBbeta(y;\,p,\,q,\,\varepsilon) = \mathrm{beta}(y;\,\varepsilon,\,\varepsilon) \cdot h(y)$, where
\begin{equation*}
    h(y) = \left[
\tfrac{1-q}{y(1-y)}
\gamma(y,p)
\right]^{\varepsilon}
\big[1-4q\,\gamma(y,p)\big]^{-(\varepsilon + \nicefrac{1}{2})} =\frac{p^\varepsilon(1-p)^\varepsilon}{(p(1-y)+(1-p)y)^{2\varepsilon}}
    \cdot \frac{(1-q)^\varepsilon}{(1-4q\gamma(y,p))^{\varepsilon+1/2}}.
\end{equation*}
Note that $h$ is continuous, strictly positive, and bounded on $[0,1]$,
so the boundary behavior of $f(y)$ is inherited entirely from the
$\mathrm{beta}(\varepsilon,\varepsilon)$ kernel $y^{\varepsilon-1}(1-y)^{\varepsilon-1}$.

\medskip
\noindent\textit{Part (1).} For $\varepsilon > 1$, the kernel satisfies
$y^{\varepsilon-1}(1-y)^{\varepsilon-1} \to 0$ as $y \to 0^+$ and $y \to 1^-$, so
$f(y) \to 0$ at both endpoints.

\medskip
\noindent\textit{Part (2).} For $\varepsilon < 1$, the kernel satisfies
$y^{\varepsilon-1}(1-y)^{\varepsilon-1} \to +\infty$ as $y \to 0^+$ and $y \to 1^-$. Since
$h$ is bounded away from zero, $f(y) \to +\infty$ at both endpoints, establishing
modes at $0$ and $1$. To see that an interior mode can additionally exist, take
$p = \nicefrac{1}{2}$, under which $f$ is symmetric about $y = \nicefrac{1}{2}$, making
it always a critical point. $\gamma\big(y,\,\nicefrac{1}{2}\big) = y(1-y)$ so $\ell(y) = (\varepsilon-1)\log(y) + (\varepsilon-1)\log(1-y) + \log(1-q) - (\varepsilon+\nicefrac{1}{2})\log\big(1-4qy(1-y)\big)$.

Computing the second derivative of $\log f$ at
$y = \nicefrac{1}{2}$ gives
\begin{align*}
    &\ell''\!\left(\tfrac{1}{2}\right) = -8(\varepsilon-1) - 8q\frac{\varepsilon + \frac{1}{2}}{1-q}\\
    &\ell''\!\left(\tfrac{1}{2}\right) < 0
    \quad\Longleftrightarrow\quad
    q > \frac{2(1-\varepsilon)}{3},
\end{align*}
so $y = \tfrac{1}{2}$ is an interior mode whenever this condition holds.

\medskip
\noindent\textit{Part (3).} For $\varepsilon = 1$, the beta kernel is $y^0(1-y)^0 = 1$, so $f(y) = h(y)$ is continuous and strictly positive on $[0,1]$, including at the boundaries. Evaluating directly at $y \teq 0$: $D\big|_{y=0} = p$, $\gamma(0,p) = 0$, and
\begin{equation*}
    \TNB(0;\,p,\,q,\,1) = \frac{p(1\tm p)}{p^2}\cdot\frac{(1\tm q)}{1} = \frac{(1\tm p)(1\tm q)}{p}.
\end{equation*}
Similarly at $y \teq 1$: $D\big|_{y=1} = 1\tm p$, $\gamma(1,p) = 0$, and
\begin{equation*}
    \TNB(1;\,p,\,q,\,1) = \frac{p(1\tm p)}{(1\tm p)^2}\cdot\frac{(1\tm q)}{1} = \frac{p(1\tm q)}{1\tm p}.
\end{equation*}
\end{proof}

\restatealiasOn
\noindent\textbf{\Cref{cor:tilt}} (\corTiltTitle). {\itshape\corTiltBody}
\restatealiasOff
\begin{proof}
The Libby-Novick beta density is
\begin{equation*} \mathrm{LNbeta}\Big(y;\,\varepsilon,\,\varepsilon,\,\tfrac{1-p}{p}\Big) = \frac{y^{\varepsilon-1}(1-y)^{\varepsilon-1}}{B(\varepsilon,\varepsilon)}\cdot\frac{p^\varepsilon(1\tm p)^\varepsilon}{D^{2\varepsilon}}
\end{equation*}
where $D = p(1\tm y) + (1\tm p)y$. Dividing the TNBbeta density in~\Cref{eq:pdf} by this expression leaves the factor $(1\tm q)^\varepsilon(1 - 4q\gamma(y,p))^{-(\varepsilon+1/2)}$, which equals $1$ when $q = 0$.
\end{proof}

%%%%%%%%%%%%%%%%%%%%%%%%%%%%%%%%%%%%%%%%%%%%%%%%%%%%%%%%%%%
% Appendix B: Proofs for the Negative Binomial Mixing Distributions
%%%%%%%%%%%%%%%%%%%%%%%%%%%%%%%%%%%%%%%%%%%%%%%%%%%%%%%%%%%
\section{Proofs for~\Cref{sec:mixing}}\label{app:proof2}

\begin{lemma}[\textbf{General NB-beta marginalization}]\label{lemma:general_lnb}
Let $\alpha_1,\,\alpha_2 > 0$ and $p_1,\,p_2 \in (0,1)$. Define the following auxiliary-variable randomization of a standard beta random variable
\begin{equation*}
\begin{aligned}
&J_1 \sim \mathrm{NB}(\alpha_1,\,p_1), \qquad J_2 \sim \mathrm{NB}(\alpha_2,\,p_2),\\
&Y \mid J_1 \teq j_1,\, J_2 \teq j_2 \sim \mathrm{beta}\big(\alpha_1 \tp j_1,\,\alpha_2 \tp j_2\big).
\end{aligned}
\end{equation*}
Then the marginal distribution is $Y \sim \mathrm{LNbeta}\big(\alpha_1,\,\alpha_2,\, \nicefrac{p_1}{p_2}\big)$.
\end{lemma}
\begin{proof}
We jointly marginalize $J_1$ and $J_2$. Expanding the beta and negative binomial densities and cancelling $\Gamma(\alpha_i + j_i)$ terms:
\begin{equation*}
    f(y) = \frac{y^{\alpha_1 - 1}(1-y)^{\alpha_2-1}}{B(\alpha_1,\alpha_2)}\,p_1^{\alpha_1}p_2^{\alpha_2}\sum_{j_1=0}^\infty \sum_{j_2=0}^\infty \frac{\Gamma(\alpha_1+\alpha_2+j_1+j_2)}{\Gamma(\alpha_1 +\alpha_2)\,j_1!\,j_2!}\big(y(1-p_1)\big)^{j_1}\big((1-y)(1-p_2)\big)^{j_2}.
\end{equation*}
Re-indexing with $s = j_1 + j_2$ and applying the binomial theorem to the inner sum:
\begin{align*}
    &\sum_{s=0}^\infty \frac{\Gamma(\alpha_1+\alpha_2+s)}{\Gamma(\alpha_1 +\alpha_2)\,s!}\sum_{j_1=0}^s \binom{s}{j_1}\big(y(1-p_1)\big)^{j_1}\big((1-y)(1-p_2)\big)^{s-j_1}\\
    &\qquad= \sum_{s=0}^\infty \frac{\Gamma(\alpha_1+\alpha_2+s)}{\Gamma(\alpha_1 +\alpha_2)\,s!}\big(y(1-p_1) + (1-y)(1-p_2)\big)^s.
\end{align*}
Closing the series with the identity $\sum_{s=0}^\infty \frac{\Gamma(a+s)}{\Gamma(a)\,s!}x^s = (1-x)^{-a}$ and simplifying:
\begin{equation*}
    f(y) = \frac{y^{\alpha_1-1}(1-y)^{\alpha_2-1}}{B(\alpha_1,\alpha_2)}\frac{p_1^{\alpha_1}p_2^{\alpha_2}}{\big(p_2 - (p_2-p_1)y\big)^{\alpha_1+\alpha_2}} = \frac{y^{\alpha_1-1}(1-y)^{\alpha_2-1}}{B(\alpha_1,\alpha_2)}\frac{c^{\alpha_1}}{\big(1 - (1 - c)y\big)^{\alpha_1+\alpha_2}}
\end{equation*}
where $c=\nicefrac{p_1}{p_2}$. This is the Libby-Novick beta density $\mathrm{LNbeta}(\alpha_1,\,\alpha_2,\,c)$, as in~\Cref{def:lnb}.
\end{proof}

\newpage

\restatealiasOn
\noindent\textbf{\Cref{thm:triple}} (\thmTripleTitle). {\itshape\thmTripleBody}
\restatealiasOff
\begin{proof}
By~\Cref{lemma:general_lnb} with $\alpha_1 = \alpha_2 = \varepsilon + c$, $p_1 = 1\tm p$, and $p_2 = p$, marginalizing $(A,\,B)$ for fixed $C\teq c$ gives $Y \mid C \teq c \sim \mathrm{LNbeta}\big(\varepsilon + c,\,\varepsilon + c,\,\tfrac{1-p}{p}\big)$ with density
\begin{equation*}
    f(y \mid c) = \frac{y^{\varepsilon+c-1}(1-y)^{\varepsilon+c-1}}{B(\varepsilon+c,\,\varepsilon+c)}\cdot\frac{p^{\varepsilon+c}(1\tm p)^{\varepsilon+c}}{D^{2(\varepsilon+c)}}
\end{equation*}
where $D = p(1\tm y) + (1\tm p)y$. Marginalizing $C \sim \mathrm{NB}(\varepsilon,\,1\tm q)$:
\begin{align*}
    f(y) &= \sum_{c=0}^\infty \mathrm{LNbeta}\big(y;\, \varepsilon \tp c,\,\varepsilon \tp c,\,\tfrac{1-p}{p}\big)\,\frac{\Gamma(\varepsilon + c)}{\Gamma(\varepsilon)\,c!}(1\tm q)^\varepsilon q^c\\
    &= \frac{y^{\varepsilon-1}(1-y)^{\varepsilon-1}\,p^\varepsilon(1\tm p)^\varepsilon}{D^{2\varepsilon}}\cdot(1\tm q)^\varepsilon\sum_{c=0}^\infty \frac{\Gamma(\varepsilon+c)}{\Gamma(\varepsilon)\,c!}\cdot\frac{\Gamma(2\varepsilon+2c)}{\Gamma(\varepsilon+c)^2}\cdot\left(\frac{y(1\tm y)p(1\tm p)}{D^2}\,q\right)^c
\end{align*}
where we have factored out terms independent of $c$. We simplify $\Gamma(2\varepsilon+2c)/\Gamma(\varepsilon+c)$ via the Legendre duplication formula $\Gamma(2z) = 2^{2z-1}\pi^{-1/2}\,\Gamma(z)\,\Gamma(z+\tfrac{1}{2})$:
\begin{equation*}
    \frac{\Gamma(2\varepsilon+2c)}{\Gamma(\varepsilon+c)} = \frac{2^{2\varepsilon+2c-1}}{\sqrt{\pi}}\,\Gamma\!\left(\varepsilon + c + \tfrac{1}{2}\right).
\end{equation*}
Substituting and writing $\gamma(y,p) = \nicefrac{y(1\tm y)p(1\tm p)}{D^2}$:
\begin{align*}
    f(y) &= \frac{y^{\varepsilon-1}(1-y)^{\varepsilon-1}\,p^\varepsilon(1\tm p)^\varepsilon}{D^{2\varepsilon}}\cdot(1\tm q)^\varepsilon\cdot\frac{2^{2\varepsilon-1}}{\sqrt{\pi}\,\Gamma(\varepsilon)}\sum_{c=0}^\infty \frac{\Gamma(\varepsilon+c+\tfrac{1}{2})}{c!}\,\big(4q\gamma(y,p)\big)^c.
\end{align*}
The series is $\sum_{c=0}^\infty \frac{\Gamma(\varepsilon+\frac{1}{2}+c)}{c!}(4q\gamma)^c = \Gamma\!\left(\varepsilon + \tfrac{1}{2}\right)\big(1 - 4q\gamma(y,p)\big)^{-(\varepsilon+1/2)}$. Therefore
\begin{equation*}
    f(y) = \frac{y^{\varepsilon-1}(1-y)^{\varepsilon-1}\,p^\varepsilon(1\tm p)^\varepsilon}{D^{2\varepsilon}}\cdot(1\tm q)^\varepsilon\cdot\frac{2^{2\varepsilon-1}\,\Gamma(\varepsilon+\tfrac{1}{2})}{\sqrt{\pi}\,\Gamma(\varepsilon)}\cdot(1 - 4q\gamma)^{-(\varepsilon+1/2)}.
\end{equation*}
Applying the duplication formula once more gives $\frac{2^{2\varepsilon-1}\,\Gamma(\varepsilon+\frac{1}{2})}{\sqrt{\pi}\,\Gamma(\varepsilon)} = \frac{\Gamma(2\varepsilon)}{\Gamma(\varepsilon)^2} = \frac{1}{B(\varepsilon,\varepsilon)}$, so
\begin{equation*}
    f(y) = \frac{y^{\varepsilon-1}(1-y)^{\varepsilon-1}}{B(\varepsilon,\varepsilon)}\cdot\frac{p^\varepsilon(1\tm p)^\varepsilon}{D^{2\varepsilon}}\cdot\frac{(1\tm q)^\varepsilon}{(1 - 4q\gamma(y,p))^{\varepsilon+1/2}} = \TNB(y;\,p,\,q,\,\varepsilon). \qedhere
\end{equation*}
\end{proof}

\restatealiasOn
\noindent\textbf{\Cref{cor:lnb_nb}} (\corLnbNbTitle). {\itshape\corLnbNbBody}
\restatealiasOff
\begin{proof}
    The result follows directly from~\Cref{lemma:general_lnb} with specific parameter values.
\end{proof}

\restatealiasOn
\noindent\textbf{\Cref{cor:K}} (\corKTitle). {\itshape\corKBody}
\restatealiasOff

\begin{proof}
By~\Cref{thm:triple}, the marginal of $Y$ over $(C,A,B)$ is $\TNB(p,\,q,\,\varepsilon)$. Marginalizing only $(A,\,B)$ for fixed $C\teq c$ is the construction in~\Cref{cor:lnb_nb} with $\varepsilon$ replaced by $\varepsilon + c$, giving $Y \mid C \teq c \sim \mathrm{LNbeta}\big(\varepsilon+c,\,\varepsilon+c,\,\tfrac{1-p}{p}\big)$.
\end{proof}
\newpage
\restatealiasOn
\noindent\textbf{\Cref{prop:gen}} (\propGenTitle). {\itshape\propGenBody}
\restatealiasOff
\begin{proof}
Since $D = A + C$ and $E = B + C$, and $A$ and $B$ are independent given $C$, we marginalize $C$ noting that $D \teq d$ and $E \teq e$ constrain $C \leq d \wedge e$:
\begin{equation*}
    P(D \teq d,\, E \teq e) = \sum_{c=0}^{d \wedge e} P(A \teq d \tm c \mid C \teq c)\,P(B \teq e \tm c \mid C \teq c)\,P(C \teq c).
\end{equation*}
Expanding each negative binomial PMF in Gamma function form:
\begin{align*}
    P(A \teq d \tm c \mid C \teq c) &= \frac{\Gamma(\varepsilon + d)}{\Gamma(\varepsilon+c)\,(d - c)!}\,(1\tm p)^{\varepsilon+c}\,p^{d-c},\\
    P(B \teq e \tm c \mid C \teq c) &= \frac{\Gamma(\varepsilon + e)}{\Gamma(\varepsilon+c)\,(e - c)!}\,p^{\varepsilon+c}\,(1\tm p)^{e-c},\\
    P(C \teq c) &= \frac{\Gamma(\varepsilon + c)}{\Gamma(\varepsilon)\,c!}\,(1\tm q)^\varepsilon\,q^c.
\end{align*}
The $p$ and $(1\tm p)$ terms combine as $(1\tm p)^{\varepsilon+c}\cdot p^{d-c}\cdot p^{\varepsilon+c}\cdot(1\tm p)^{e-c} = p^{\varepsilon+d}(1\tm p)^{\varepsilon+e}$, which is independent of $c$. One factor of $\Gamma(\varepsilon + c)$ cancels between the numerator of $P(C\teq c)$ and the denominator of $P(A \teq d\tm c \mid C\teq c)$. Factoring out all terms independent of $c$:
\begin{align*}
    P(D \teq d,\,E \teq e) &= \frac{\Gamma(\varepsilon+d)\,\Gamma(\varepsilon+e)}{\Gamma(\varepsilon)}\,p^{\varepsilon+d}(1\tm p)^{\varepsilon+e}(1\tm q)^\varepsilon\sum_{c=0}^{d \wedge e}\frac{q^c}{(d-c)!\,(e-c)!\,\Gamma(\varepsilon+c)\,c!}.
\end{align*}
To evaluate the sum, we use the Pochhammer identity $1/(m\tm c)! = (-1)^c(-m)_c/m!$ so
\begin{equation*}
    \frac{1}{(d\tm c)!\,(e\tm c)!\,\Gamma(\varepsilon+c)\,c!} = \frac{(-d)_c\,(-e)_c}{d!\,e!\,\Gamma(\varepsilon)\,(\varepsilon)_c\,c!}
\end{equation*}
where $(-1)^{2c} = 1$. Last, recognize the Gauss hypergeometric series and the negative binomial mass functions $\tbinom{\varepsilon+d-1}{d}(1\tm p)^\varepsilon p^{d} = \mathrm{NB}(d;\,\varepsilon,\,1\tm p)$ and $\tbinom{\varepsilon+e-1}{e}p^\varepsilon(1\tm p)^{e} = \mathrm{NB}(e;\,\varepsilon,\,p)$ so
\begin{equation*}
    P(D \teq d,\,E \teq e) = \mathrm{NB}(d;\,\varepsilon,\,1\tm p)\cdot\mathrm{NB}(e;\,\varepsilon,\,p)\cdot(1\tm q)^\varepsilon\;{}_2F_1(-d,\,-e;\,\varepsilon;\,q). \qedhere
\end{equation*}
\end{proof}

\restatealiasOn
\noindent\textbf{\Cref{prop:con}} (\propConTitle). {\itshape\propConBody}
\restatealiasOff
\begin{proof}
We begin with the second statement and keep only terms proportional to $a$ to write
\begin{align*}
    P\big(A \teq a \mid B \teq b,\, Y \teq y\big) &\propto \mathrm{beta}\big(y;\; \varepsilon + a,\, \varepsilon + b\big)\cdot\mathrm{NB}\big(a;\,\varepsilon,\,1- p\big)\\
    &\propto \frac{\Gamma(2\varepsilon + b + a)}{a!}\big(yp\big)^{a}
\end{align*}
which is the kernel of $\mathrm{NB}\big(2\varepsilon + b,\, 1-yp\big)$.

For the first statement, we write the joint posterior over both counts. By Bayes' rule,
\begin{align*}
    P(A \teq a,\,B \teq b \mid Y \teq y) 
    &\propto \mathrm{beta}\big(y;\,\varepsilon\tp a,\,\varepsilon\tp b\big)\cdot\mathrm{NB}\big(a;\,\varepsilon,\,1\tm p\big)\cdot\mathrm{NB}\big(b;\,\varepsilon,\,p\big)\\
    &\propto \frac{\Gamma(2\varepsilon + a + b)}{a!\,b!}\,\big(yp\big)^{a}\,\big((1\tm y)(1\tm p)\big)^{b}
\end{align*}
Then marginalize over $B$ to form the posterior marginal of $A$ as
\begin{equation*}
    P(A \teq a \mid Y \teq y) \propto \frac{\big(yp\big)^{a}}{a!}\sum_{b=0}^\infty\frac{\Gamma(2\varepsilon + a + b)}{ b!}\big((1-y)(1-p)\big)^{b}.
\end{equation*}
Finally, we use the series identity $\sum_{j=0}^\infty \frac{\Gamma(\alpha+j)}{j!}x^j = \Gamma(\alpha)(1-x)^{-\alpha}$ to write
\begin{align*}
    P(A \teq a \mid Y \teq y) &\propto \frac{\Gamma(2\varepsilon + a)}{a!}\cdot\frac{\big(yp\big)^{a}}{\big(1-(1-y)(1-p)\big)^{2\varepsilon+a}}\\
    &\propto \frac{\Gamma(2\varepsilon + a)}{a!}\left(\frac{yp}{1-(1-y)(1-p)}\right)^{a}
\end{align*}
which is the kernel of $\mathrm{NB}\!\left(2\varepsilon,\,1 \tm \frac{yp}{1-(1-y)(1-p)}\right)$.
\end{proof}

\restatealiasOn
\noindent\textbf{\Cref{prop:consum}} (\propConsumTitle). {\itshape\propConsumBody}
\restatealiasOff
\begin{proof}
For the first statement, begin from the joint inverse distribution
\begin{equation*}
    P(A \teq a,\,B \teq b \mid Y \teq y) \propto \frac{\Gamma(2\varepsilon + a + b)}{a!\,b!}\,\big(yp\big)^{a}\,\big((1\tm y)(1\tm p)\big)^{b}.
\end{equation*}
Substituting $b = s \tm a$ and summing over $a = 0,\ldots,s$:
\begin{align*}
    P\big(A + B \teq s \mid Y \teq y\big) &\propto \sum_{a=0}^{s}
     \frac{\Gamma(2\varepsilon + s)}{a!(s-a)!}\,\big(yp\big)^{a}\big((1\tm y)(1\tm p)\big)^{s-a}\\
     &\propto \frac{\Gamma(2\varepsilon + s)}{s!}
    \sum_{a=0}^{s}\binom{s}{a}\big(yp\big)^{a}\big((1\tm y)(1\tm p)\big)^{s-a}.
\end{align*}
where we used $\binom{s}{a} = s!/[a!(s\tm a)!]$. Applying the binomial theorem gives
\begin{equation*}
    P\big(A + B \teq s \mid Y \teq y\big) \propto \frac{\Gamma(2\varepsilon + s)}{s!}
    \big(yp + (1-y)(1-p)\big)^{s}
\end{equation*}
which is the kernel of $\mathrm{NB}\big(2\varepsilon,\, p(1-y) + y(1-p)\big)$.

For the second statement, we write the conditional as a ratio of the joint and marginal:
\begin{equation*}
    P\big(A \teq a \mid A + B \teq s,\,Y \teq y\big) = \frac{P(A \teq a,\,B \teq s \tm a \mid Y \teq y)}{P(A + B \teq s \mid Y \teq y)}.
\end{equation*}
Substituting the expressions above and cancelling the common factor $\Gamma(2\varepsilon+s)$:
\begin{equation*}
    P\big(A \teq a \mid A + B \teq s,\,Y \teq y\big) \propto \binom{s}{a}\big(yp\big)^{a}\big((1-y)(1-p)\big)^{s-a}
\end{equation*}
which is the kernel of $\mathrm{binomial}\!\left(s,\,\nicefrac{py}{py+(1-p)(1-y)}\right)$.
\end{proof}

\restatealiasOn
\noindent\textbf{\Cref{prop:Kconditional}} (\propKconditionalTitle). {\itshape\propKconditionalBody}
\restatealiasOff
\begin{proof}
By~\Cref{cor:K}, $Y \mid C \teq c \sim \mathrm{LNbeta}\big(\varepsilon+c,\,\varepsilon+c,\,\tfrac{1-p}{p}\big)$ and $C \sim \mathrm{NB}(\varepsilon,\,1\tm q)$. By Bayes' rule,
\begin{align*}
    P(C \teq c \mid Y \teq y) &\propto \mathrm{LNbeta}\Big(y;\; \varepsilon \tp c,\,\varepsilon\tp c,\,\tfrac{1-p}{p}\Big)\cdot \mathrm{NB}\big(c\; \varepsilon,\, 1\tm q\big)\\
     &\propto \frac{1}{B(\varepsilon\tp c,\,\varepsilon\tp c)}\cdot\frac{\big(y(1\tm y)p(1\tm p)\big)^c}{\big(p(1\tm y) + (1\tm p)y\big)^{2c}}\cdot\frac{\Gamma(\varepsilon\tp c)}{c!}\,q^c\\
     &\propto \frac{\Gamma(2\varepsilon+2c)}{\Gamma(\varepsilon+c)}\cdot\frac{\big(\gamma(y,p) q\big)^c}{c!}
\end{align*}
where we recognize the similarity function $\gamma(y,p) = \nicefrac{y(1\tm y)p(1\tm p)}{\big(p(1\tm y) + (1\tm p)y\big)^2}$ Applying the Legendre duplication formula
$\Gamma(2z) = 2^{2z-1}\pi^{-1/2}\,\Gamma(z)\,\Gamma(z\tp\tfrac{1}{2})$ with $z = \varepsilon \tp c$ gives
\begin{equation*}
    P(C \teq c \mid Y \teq y) \propto \frac{\Gamma(\varepsilon + \tfrac{1}{2} + c)}{c!}\,\big(4q\gamma(y,p)\big)^c
\end{equation*}
which is the kernel of $\mathrm{NB}\big(\varepsilon + \tfrac{1}{2},\,1 \tm 4q\gamma(y,p)\big)$.
\end{proof}

\section{Experimental Details}\label{sec:app_exp}

We provide additional dataset and computational details for the experiments in~\Cref{sec:experiments}. For the model implementations in each experiment, we use Stan~\citep{carpenter_stan_2017} for all beta regression models and the code provided by~\cite{lee2026scalable} for cobin and micobin models. We modify the micobin code for ICAR random effects for the experiments in~\Cref{sec:trees}. To implement TNBbeta models, we use existing Pólya-gamma samplers~\citep{polson_bayesian_2013,windle_sampling_2014}.

\subsection{\Cref{sec:bench} Details}\label{sec:app_datasets}

\Cref{tab:datasets} summarizes the seven datasets used in the experiments of~\Cref{sec:bench}.
All predictors are centered and standardized prior to fitting, and an intercept column is appended.
A random 10\% holdout set is used for predictive evaluation in each model fit.

The two synthetic datasets are generated from a beta regression model with $Y_i \sim \textrm{beta}(\mu_i \phi,\, (1-\mu_i)\phi)$, $\mu_i = \textrm{logit}^{-1}(X_i^\top \beta)$, $\phi = 5$, and $\beta_j \sim \mathcal{N}(0, 0.2)$ for each coefficient including the intercept.
The orthogonal design matrix is constructed via QR decomposition of a Gaussian matrix.
The collinear design matrix is constructed from a 5-factor Gaussian factor model with additive noise.

\begin{table}[ht]
\centering
\caption{Datasets used in the~\Cref{sec:bench} experiments. $n$ is the number of observations and $p$ is the number of predictors (excluding the intercept).}
\label{tab:datasets}
\small
\begin{tabular}{llrrl}
\toprule
Dataset & Response $Y$ & $n$ & $p$ & Source \\
\midrule
AlcoholUse & Alcohol use percentage & 1{,}340 & 3 & \texttt{zoib} R package \\
Bike & Casual / total rentals & 731 & 11 & UCI ML Repository (ID 275) \\
Credit & Recent payment ratio & 18{,}150 & 11 & UCI ML Repository (ID 350) \\
Crime & Violent crimes per capita & 1{,}940 & 20 & UCI ML Repository (ID 183) \\
Productivity & Actual productivity & 1{,}160 & 10 & UCI ML Repository (ID 597) \\
Synthetic (orth.) & Simulated beta & 500 & 20 & Generated \\
Synthetic (corr.) & Simulated beta & 500 & 20 & Generated \\
\bottomrule
\end{tabular}
\end{table}

\Cref{tab:ess_single} reports the effective sample size and wall-clock time for each model in the shared concentration experiment. Furthermore,~\Cref{tab:bench_dispreg} reports the information rate, effective sample size, ESS per second, and wall-clock time for the concentration regression experiment. Last,~\Cref{tab:bench_nostd} shows the results in the shared concentration setting on data without covariate standardization, which can have a large negative effect on the computational efficiency of beta regression via HMC while the results for the TNBbeta are largely unchanged.

\begin{table}[ht]
\centering
\caption{ESS and wall-clock time (seconds) for shared concentration models.}
\label{tab:ess_single}
% Auto-generated by export_results.R
% Do not edit manually.

\small
\begin{tabular}{l cc cc cc cc}
\toprule
  & \multicolumn{2}{c}{TNBbeta} & \multicolumn{2}{c}{Beta} & \multicolumn{2}{c}{Cobin} & \multicolumn{2}{c}{Micobin} \\
 \cmidrule(lr){2-3} \cmidrule(lr){4-5} \cmidrule(lr){6-7} \cmidrule(lr){8-9}
Dataset & ESS & Time (s) & ESS & Time (s) & ESS & Time (s) & ESS & Time (s) \\
\midrule
Orthogonal & 905 \scriptsize{(4)} & 2.5 & 4655 \scriptsize{(66)} & 3.7 & 1389 \scriptsize{(10)} & 6.5 & 1003 \scriptsize{(4)} & 15.0 \\
Collinear & 945 \scriptsize{(5)} & 2.7 & 2981 \scriptsize{(71)} & 17.1 & 1679 \scriptsize{(11)} & 6.5 & 1169 \scriptsize{(6)} & 15.8 \\
Bike & 677 \scriptsize{(4)} & 2.5 & 1764 \scriptsize{(28)} & 27.5 & 763 \scriptsize{(7)} & 18.5 & 483 \scriptsize{(4)} & 40.5 \\
Product & 952 \scriptsize{(6)} & 6.0 & 2703 \scriptsize{(34)} & 11.4 & 1221 \scriptsize{(10)} & 13.2 & 775 \scriptsize{(9)} & 41.6 \\
Alcohol & 681 \scriptsize{(11)} & 6.8 & 1811 \scriptsize{(19)} & 6.1 & 173 \scriptsize{(4)} & 18.0 & 168 \scriptsize{(2)} & 46.8 \\
Crime & 851 \scriptsize{(4)} & 11.0 & 1789 \scriptsize{(19)} & 127.5 & 1056 \scriptsize{(6)} & 21.6 & 737 \scriptsize{(4)} & 58.4 \\
Credit & 954 \scriptsize{(5)} & 93.4 & 2595 \scriptsize{(39)} & 138.2 & 428 \scriptsize{(2)} & 113.8 & 420 \scriptsize{(2)} & 404.1 \\
\bottomrule
\end{tabular}

\end{table}

\begin{table}[ht]
\centering
\caption{TNBbeta regression models with covariates on the concentration parameter tend to match or improve on prediction and efficiency of the analogous beta models.}
\label{tab:bench_dispreg}
% Auto-generated by export_results.R
% Do not edit manually.

\small
\setlength{\tabcolsep}{3pt}
\begin{tabular}{l cc cccc cccc}
\toprule
 & &  & \multicolumn{4}{c}{TNBbeta} & \multicolumn{4}{c}{Beta} \\
 \cmidrule(lr){4-7} \cmidrule(lr){8-11}
Dataset & $n$ & $p$ & IR $(\downarrow)$ & ESS & sec & $\nicefrac{\textrm{ESS}}{\textrm{sec}}$ & IR $(\downarrow)$ & ESS & sec & $\nicefrac{\textrm{ESS}}{\textrm{sec}}$ \\
\midrule
Orthogonal & 500 & 20 & -0.31 \scriptsize{(0.02)} & 495 \scriptsize{(9)} & 3.3 & 149 & \textbf{-0.41 \scriptsize{(0.02)}} & 2407 \scriptsize{(39)} & 5.2 & \textbf{462} \\[2pt]
Collinear & 500 & 20 & \textbf{-0.29 \scriptsize{(0.02)}} & 715 \scriptsize{(4)} & 4.1 & \textbf{174} & \textbf{-0.31 \scriptsize{(0.02)}} & 3380 \scriptsize{(47)} & 25.5 & 133 \\[2pt]
Bike & 731 & 11 & \textbf{-1.65 \scriptsize{(0.02)}} & 586 \scriptsize{(6)} & 5.4 & \textbf{109} & \textbf{-1.64 \scriptsize{(0.03)}} & 1945 \scriptsize{(52)} & 30.6 & 64 \\[2pt]
Product & 1,160 & 10 & \textbf{-0.94 \scriptsize{(0.02)}} & 770 \scriptsize{(16)} & 7.5 & \textbf{103} & -0.65 \scriptsize{(0.03)} & 1698 \scriptsize{(36)} & 21.4 & 79 \\[2pt]
Alcohol & 1,288 & 3 & -2.26 \scriptsize{(0.02)} & 496 \scriptsize{(10)} & 10.4 & 48 & \textbf{-2.31 \scriptsize{(0.02)}} & 2111 \scriptsize{(37)} & 7.5 & \textbf{281} \\[2pt]
Crime & 1,940 & 20 & \textbf{-1.00 \scriptsize{(0.02)}} & 769 \scriptsize{(6)} & 19.1 & \textbf{40} & \textbf{-0.97 \scriptsize{(0.02)}} & 2010 \scriptsize{(27)} & 187.9 & 11 \\[2pt]
Credit & 18,150 & 11 & \textbf{-1.35 \scriptsize{(0.01)}} & 656 \scriptsize{(5)} & 152.6 & 4 & -1.03 \scriptsize{(0.01)} & 2331 \scriptsize{(30)} & 295.3 & \textbf{8} \\
\bottomrule
\end{tabular}

\end{table}

\begin{table}
\centering
\caption{Shared concentration results without covariate standardization. HMC efficiency is sensitive to the magnitude of the covariates.}
\label{tab:bench_nostd}
% Auto-generated by export_results.R
% Do not edit manually.

\small
\setlength{\tabcolsep}{3pt}
\begin{tabular}{l cc cc cc cc cc}
\toprule
 & &  & \multicolumn{2}{c}{TNBbeta} & \multicolumn{2}{c}{Beta} & \multicolumn{2}{c}{Cobin} & \multicolumn{2}{c}{Micobin} \\
 \cmidrule(lr){4-5} \cmidrule(lr){6-7} \cmidrule(lr){8-9} \cmidrule(lr){10-11}
Dataset & $n$ & $p$ & IR $(\downarrow)$ & $\nicefrac{\textrm{ESS}}{\textrm{sec}}$ & IR $(\downarrow)$ & $\nicefrac{\textrm{ESS}}{\textrm{sec}}$ & IR $(\downarrow)$ & $\nicefrac{\textrm{ESS}}{\textrm{sec}}$ & IR $(\downarrow)$ & $\nicefrac{\textrm{ESS}}{\textrm{sec}}$ \\
\midrule
Orthogonal & 500 & 20 & -0.35 \scriptsize{(0.02)} & 368 & \textbf{-0.42 \scriptsize{(0.02)}} & \textbf{1105} & -0.32 \scriptsize{(0.03)} & 211 & -0.35 \scriptsize{(0.02)} & 64 \\[2pt]
Collinear & 500 & 20 & \textbf{-0.31 \scriptsize{(0.02)}} & \textbf{352} & \textbf{-0.33 \scriptsize{(0.02)}} & 169 & \textbf{-0.31 \scriptsize{(0.02)}} & 253 & \textbf{-0.31 \scriptsize{(0.02)}} & 72 \\[2pt]
Bike & 731 & 11 & \textbf{-1.60 \scriptsize{(0.02)}} & \textbf{289} & \textbf{-1.58 \scriptsize{(0.02)}} & 36 & -1.45 \scriptsize{(0.02)} & 57 & -1.48 \scriptsize{(0.02)} & 18 \\[2pt]
Product & 1,160 & 10 & \textbf{-0.67 \scriptsize{(0.01)}} & \textbf{161} & -0.56 \scriptsize{(0.01)} & $<$1 & -0.54 \scriptsize{(0.01)} & 99 & -0.61 \scriptsize{(0.02)} & 19 \\[2pt]
Alcohol & 1,288 & 3 & -2.18 \scriptsize{(0.02)} & \textbf{103} & \textbf{-2.30 \scriptsize{(0.02)}} & 99 & \textbf{-2.31 \scriptsize{(0.02)}} & 13 & \textbf{-2.31 \scriptsize{(0.01)}} & 4 \\[2pt]
Crime & 1,940 & 20 & \textbf{-0.99 \scriptsize{(0.02)}} & \textbf{98} & -0.88 \scriptsize{(0.02)} & 7 & -0.92 \scriptsize{(0.02)} & 70 & -0.90 \scriptsize{(0.02)} & 21 \\[2pt]
Credit & 18,150 & 11 & \textbf{-1.28 \scriptsize{(0.01)}} & \textbf{11} & -0.57 \scriptsize{(0.00)} & $<$1 & -1.17 \scriptsize{(0.01)} & 4 & -1.17 \scriptsize{(0.01)} & 1 \\
\bottomrule
\end{tabular}

\end{table}

\subsection{\Cref{sec:trees} Details}\label{sec:app_spatial}

\Cref{tab:covariates} describes the six environmental covariates associated with each site in the tree canopy dataset of~\Cref{sec:trees}.
All covariates are centered and standardized prior to fitting, and an intercept is appended, giving $p=7$ columns in the design matrix.

\begin{table}[ht]
\centering
\caption{Environmental covariates for the tree canopy dataset. Each covariate is computed as the average within the corresponding $20 \!\times\! 20$ meter cell.}
\label{tab:covariates}
\small
\begin{tabular}{ll}
\toprule
Covariate & Description \\
\midrule
\texttt{wetness} & Topographic wetness index \\
\texttt{southness} & Aspect southness component \\
\texttt{degreedays} & Growing degree days \\
\texttt{dem} & Digital elevation (meters) \\
\texttt{slope} & Slope steepness (degrees) \\
\texttt{snowpack} & Snowpack persistence \\
\bottomrule
\end{tabular}
\end{table}

The dataset consists of a $100 \!\times\! 100$ grid of cells covering the Upper Gunnison Watershed, yielding $10{,}000$ cells.
For the beta regression comparison, we discard all sites with exactly $0\%$ canopy, leaving $N = 8{,}763$ observations as described in~\Cref{sec:trees}.
The spatial adjacency matrix uses 4-neighbor connectivity.

For the $K$-fold cross-validation experiments, we use $K = 20$ folds defined by deterministic $10 \!\times\! 10$ spatial blocks.
Each fold is fit with $4$ chains, $2{,}000$ burn-in iterations, and $1{,}000$ sampling iterations.
For the full-data fits used in~\Cref{fig:canopy}, we use $4$ chains with $5{,}000$ burn-in and $2{,}000$ sampling iterations, fit to all $10,\!000$ sites.
\Cref{tab:tree_timing} reports the MCMC sampling time and information rate computation time for each model, averaged over the $20$ cross-validation replications on identical hardware.

\begin{table}[ht]
\centering
\caption{MCMC sampling time and held-out information rate computation time for each tree canopy model, averaged over folds, in seconds.}
\label{tab:tree_timing}
% Auto-generated by export_results.R
% Do not edit manually.

\small
\setlength{\tabcolsep}{4pt}
\begin{tabular}{l cc cc cc}
\toprule
 & \multicolumn{2}{c}{TNBbeta} & \multicolumn{2}{c}{Beta (HMC)} & \multicolumn{2}{c}{Micobin} \\
\cmidrule(lr){2-3} \cmidrule(lr){4-5} \cmidrule(lr){6-7}
Model & MCMC & IR & MCMC & IR & MCMC & IR \\
\midrule
Cov + Scalar & 70 \scriptsize{(1)} & 31 \scriptsize{(2)} & 544 \scriptsize{(3)} & 12 \scriptsize{(1)} & 142 \scriptsize{(2)} & 858 \scriptsize{(29)} \\
Cov + Cov & 64 \scriptsize{(1)} & 25 \scriptsize{(2)} & 464 \scriptsize{(16)} & 16 \scriptsize{(1)} & 194 \scriptsize{(2)} & 840 \scriptsize{(33)} \\
ICAR + Scalar & 89 \scriptsize{(2)} & 17 \scriptsize{(2)} & 2009 \scriptsize{(47)} & 11 \scriptsize{(1)} & 704 \scriptsize{(19)} & 796 \scriptsize{(30)} \\
ICAR + Cov & 95 \scriptsize{(2)} & 15 \scriptsize{(2)} & 3486 \scriptsize{(170)} & 11 \scriptsize{(1)} & 664 \scriptsize{(22)} & 719 \scriptsize{(24)} \\
\bottomrule
\end{tabular}

\end{table}
