# Supplementary material for: The Triply-Randomized Negative Binomial Beta for Robust Regression and Conjugate Models of Bounded Support Data
Source: arXiv:2606.11624 source file (2026-06-10)
Supplement: Supplementary file 2 [file cor_tilt.tex]

\restatealiasOn
\noindent\textbf{\Cref{cor:tilt}} (\corTiltTitle). {\itshape\corTiltBody}
\restatealiasOff
\begin{proof}
The Libby-Novick beta density is
\begin{equation*} \mathrm{LNbeta}\Big(y;\,\varepsilon,\,\varepsilon,\,\tfrac{1-p}{p}\Big) = \frac{y^{\varepsilon-1}(1-y)^{\varepsilon-1}}{B(\varepsilon,\varepsilon)}\cdot\frac{p^\varepsilon(1\tm p)^\varepsilon}{D^{2\varepsilon}}
\end{equation*}
where $D = p(1\tm y) + (1\tm p)y$. Dividing the TNBbeta density in~\Cref{eq:pdf} by this expression leaves the factor $(1\tm q)^\varepsilon(1 - 4q\gamma(y,p))^{-(\varepsilon+1/2)}$, which equals $1$ when $q = 0$.
\end{proof}
