# Supplementary material for: The Triply-Randomized Negative Binomial Beta for Robust Regression and Conjugate Models of Bounded Support Data
Source: arXiv:2606.11624 source file (2026-06-10)
Supplement: Supplementary file 3 [file prop_phi.tex]

\restatealiasOn
\noindent\textbf{\Cref{prop:phi}} (\propPhiTitle). {\itshape\propPhiBody}
\restatealiasOff
\begin{proof}
Write $f(y) \defeq TNBbeta(y;\,p,\,q,\,\varepsilon) = \mathrm{beta}(y;\,\varepsilon,\,\varepsilon) \cdot h(y)$, where
\begin{equation*}
    h(y) = \left[
\tfrac{1-q}{y(1-y)}
\gamma(y,p)
\right]^{\varepsilon}
\big[1-4q\,\gamma(y,p)\big]^{-(\varepsilon + \nicefrac{1}{2})} =\frac{p^\varepsilon(1-p)^\varepsilon}{(p(1-y)+(1-p)y)^{2\varepsilon}}
    \cdot \frac{(1-q)^\varepsilon}{(1-4q\gamma(y,p))^{\varepsilon+1/2}}.
\end{equation*}
Note that $h$ is continuous, strictly positive, and bounded on $[0,1]$,
so the boundary behavior of $f(y)$ is inherited entirely from the
$\mathrm{beta}(\varepsilon,\varepsilon)$ kernel $y^{\varepsilon-1}(1-y)^{\varepsilon-1}$.

\medskip
\noindent\textit{Part (1).} For $\varepsilon > 1$, the kernel satisfies
$y^{\varepsilon-1}(1-y)^{\varepsilon-1} \to 0$ as $y \to 0^+$ and $y \to 1^-$, so
$f(y) \to 0$ at both endpoints.

\medskip
\noindent\textit{Part (2).} For $\varepsilon < 1$, the kernel satisfies
$y^{\varepsilon-1}(1-y)^{\varepsilon-1} \to +\infty$ as $y \to 0^+$ and $y \to 1^-$. Since
$h$ is bounded away from zero, $f(y) \to +\infty$ at both endpoints, establishing
modes at $0$ and $1$. To see that an interior mode can additionally exist, take
$p = \nicefrac{1}{2}$, under which $f$ is symmetric about $y = \nicefrac{1}{2}$, making
it always a critical point. $\gamma\big(y,\,\nicefrac{1}{2}\big) = y(1-y)$ so $\ell(y) = (\varepsilon-1)\log(y) + (\varepsilon-1)\log(1-y) + \log(1-q) - (\varepsilon+\nicefrac{1}{2})\log\big(1-4qy(1-y)\big)$.

Computing the second derivative of $\log f$ at
$y = \nicefrac{1}{2}$ gives
\begin{align*}
    &\ell''\!\left(\tfrac{1}{2}\right) = -8(\varepsilon-1) - 8q\frac{\varepsilon + \frac{1}{2}}{1-q}\\
    &\ell''\!\left(\tfrac{1}{2}\right) < 0
    \quad\Longleftrightarrow\quad
    q > \frac{2(1-\varepsilon)}{3},
\end{align*}
so $y = \tfrac{1}{2}$ is an interior mode whenever this condition holds.

\medskip
\noindent\textit{Part (3).} For $\varepsilon = 1$, the beta kernel is $y^0(1-y)^0 = 1$, so $f(y) = h(y)$ is continuous and strictly positive on $[0,1]$, including at the boundaries. Evaluating directly at $y \teq 0$: $D\big|_{y=0} = p$, $\gamma(0,p) = 0$, and
\begin{equation*}
    \TNB(0;\,p,\,q,\,1) = \frac{p(1\tm p)}{p^2}\cdot\frac{(1\tm q)}{1} = \frac{(1\tm p)(1\tm q)}{p}.
\end{equation*}
Similarly at $y \teq 1$: $D\big|_{y=1} = 1\tm p$, $\gamma(1,p) = 0$, and
\begin{equation*}
    \TNB(1;\,p,\,q,\,1) = \frac{p(1\tm p)}{(1\tm p)^2}\cdot\frac{(1\tm q)}{1} = \frac{p(1\tm q)}{1\tm p}.
\end{equation*}
\end{proof}
