# Supplementary material for: The Triply-Randomized Negative Binomial Beta for Robust Regression and Conjugate Models of Bounded Support Data
Source: arXiv:2606.11624 source file (2026-06-10)
Supplement: Supplementary file 4 [file theorem_tnbebta.tex]

\restatealiasOn
\noindent\textbf{\Cref{theorem:tnbebta}} (\thmMedianTwoTitle). {\itshape\propMedianTwoBody}
\restatealiasOff
\begin{proof}
\textit{Part (1).} We first show that if $X \sim \mathrm{LNbeta}\big(\varepsilon,\,\varepsilon,\,\tfrac{1-p}{p}\big)$ then $\mathrm{median}(X) \teq p$. Define the map $x \teq g(y)$ as follows
\begin{equation*}
    x = \frac{y(1-p)}{y(1-p)+(1-y)p}
\end{equation*}
We show that this map transforms Libby-Novick beta density into the symmetric beta density $\textrm{beta}(\varepsilon,\,\varepsilon)$. Let $D = y(1-p)+(1-y)p$. Then the Jacobian is
\begin{equation*}
    \frac{dx}{dy} = \frac{(1-p)D - y(1-p)(1-2p)}{D^2} = \frac{p(1-p)}{D^2}
\end{equation*}
which is positive, so the map is strictly increasing. Under the map $g$, $x = \nicefrac{y(1-p)}{D}$ and $1-x = \nicefrac{(1-y)p}{D}$, so
\begin{equation*}
    x^{\varepsilon-1}(1-x)^{\varepsilon-1} = \frac{\big(y(1-p)\big)^{\varepsilon-1}\big((1-y)p\big)^{\varepsilon-1}}{D^{2(\varepsilon-1)}}
\end{equation*}
Therefore the change-of-variables formula $f_X(x)\,|dx/dy| = f_Y(y)$:
\begin{equation*}
    \underbrace{\frac{x^{\varepsilon-1}(1-x)^{\varepsilon-1}}{B(\varepsilon,\varepsilon)}}_{\text{beta}(\varepsilon,\varepsilon)} \cdot \frac{p(1-p)}{D^2}
    = \frac{y^{\varepsilon-1}(1-y)^{\varepsilon-1}}{B(\varepsilon,\varepsilon)} \cdot \frac{(1-p)^\varepsilon p^\varepsilon}{D^{2\varepsilon}}
\end{equation*}
which recovers the Libby-Novick beta density as desired. Now because $g(y)$ is strictly increasing, the median $m$ of $X$ satisfies
\begin{equation*}
    \mathbb{P}\big(X \le m\big) = \tfrac{1}{2} \iff \mathbb{P}\big(Z \le g(m)\big) = \tfrac{1}{2}
\end{equation*}
The median of $Z \sim \mathrm{beta}(\varepsilon,\varepsilon)$ is $\tfrac{1}{2}$ by symmetry, so $g(m) = \tfrac{1}{2}$. Solving:
\begin{align*}
    g(m) = &\frac{m(1-p)}{m(1-p)+(1-m)p} = \frac{1}{2} \\
    \Longleftrightarrow\quad&2m(1-p) = m(1-p)+(1-m)p \\
    \Longleftrightarrow\quad& m(1-p) = (1-m)p \\
    \Longleftrightarrow\quad& m = p
\end{align*}
Thus the median of the Libby-Novick beta under equality of its shapes is $p$.

Now, $Y \sim \textrm{TNBbeta}\big(p,\,q,\,\varepsilon\big)$ can be expressed as $Y \mid C\sim\textrm{LNbeta}\left(\varepsilon + C,\,\varepsilon + C,\,\tfrac{1-p}{p}\right)$ with $C \sim \textrm{NB}(\varepsilon,\,1-q)$ due to~\Cref{cor:K}. The marginal distribution of $Y$ is a mixture over distributions, each with median exactly $p$. Therefore, the median of $Y$ must also be $p$.

\textit{Part (2).} We evaluate the density at $y \teq p$. Note that
\begin{equation*}
    \gamma(p,\,p) = \frac{p(1\tm p)p(1\tm p)}{(2p(1\tm p))^2} = \frac{1}{4}.
\end{equation*}
Therefore $1 - 4q\gamma(p,p) = 1 - q$, and the density at $y \teq p$ is
\begin{align*}
    \TNB(p;\,p,\,q,\,\varepsilon) &= \mathrm{beta}(p; \varepsilon,\,\varepsilon) \cdot \big(4p(1-p)\big)^{-\varepsilon}\cdot \frac{(1\tm q)^\varepsilon}{(1\tm q)^{\varepsilon+1/2}}\\
    &= \mathrm{beta}(p; \varepsilon,\,\varepsilon) \cdot \big(4p(1-p)\big)^{-\varepsilon}\cdot (1\tm q)^{-1/2}.
\end{align*}
As $q \to 1$, $(1\tm q)^{-1/2} \to \infty$, so $\TNB(p;\,p,\,q,\,\varepsilon) \to \infty$.

\textit{Part (3).} Write the log-density as $\ell(y) = \ell_{\mathrm{LN}}(y;\,\varepsilon,\,p) + \varepsilon\log(1\tm q) - (\varepsilon \tp \tfrac{1}{2})\log(1 - 4q\gamma(y,p))$, where $\ell_{\mathrm{LN}}$ collects terms not involving $q$. The only term involving both $p$ and $q$ is $-(\varepsilon\tp\tfrac{1}{2})\log(1 - 4q\gamma)$. We first compute
\begin{equation*}
    \frac{\partial\gamma}{\partial p} = \frac{\partial}{\partial p}\frac{y(1\tm y)p(1\tm p)}{D^2} = \frac{y(1\tm y)(y \tm p)}{D^3}
\end{equation*}
where we have used $\frac{\partial D}{\partial p} = 1 - 2y$. Therefore
\begin{equation*}
    \frac{\partial^2 \ell}{\partial p\,\partial q} = \frac{4(\varepsilon \tp \tfrac{1}{2})\,\frac{\partial \gamma}{\partial p}}{\big(1 - 4q\gamma(y,p)\big)^2} = \frac{4(\varepsilon \tp \tfrac{1}{2})\,y(1\tm y)(y\tm p)}{D^3\big(1 - 4q\gamma(y,p)\big)^2}.
\end{equation*}
We must show $\mathcal{I}_{pq} = -\ex\!\left[\frac{\partial^2 \ell}{\partial p\,\partial q}\right] = 0$. Apply the change of variables $u \teq g(y) = \nicefrac{y(1\tm p)}{D}$ from part~(1). Setting $R = up \tp (1\tm u)(1\tm p)$, we have $D = p(1\tm p)/R$ and by direct calculation
\begin{equation*}
    y \tm p = \frac{p(1\tm p)(2u \tm 1)}{R},\qquad y(1\tm y) = \frac{u(1\tm u)p(1\tm p)}{R^2},\qquad \gamma(y,p) = u(1\tm u).
\end{equation*}
Substituting, the integrand simplifies to
\begin{equation*}
    \frac{y(1\tm y)(y\tm p)}{D^3(1 - 4q\gamma)^2}\,\mathrm{TNBbeta}(y;\,p,\,q,\,\varepsilon)\,dy = \frac{(1\tm q)^\varepsilon}{p(1\tm p)\,B(\varepsilon,\varepsilon)}\cdot\frac{u^\varepsilon(1\tm u)^\varepsilon(2u\tm 1)}{(1 - 4qu(1\tm u))^{\varepsilon+5/2}}\,du.
\end{equation*}
where again we have used the Jacobian $\frac{du}{dy} = \nicefrac{p(1-p)}{D^2}$. Since $u^\varepsilon(1\tm u)^\varepsilon$ and $(1 - 4qu(1\tm u))^{\varepsilon+5/2}$ are symmetric about $u \teq \tfrac{1}{2}$ while $(2u \tm 1)$ is antisymmetric, the integrand is antisymmetric about $u \teq \tfrac{1}{2}$. Therefore the integral over $[0,1]$ vanishes, giving $\mathcal{I}_{pq} = 0$.
\end{proof}
