# Supplementary material for: The Triply-Randomized Negative Binomial Beta for Robust Regression and Conjugate Models of Bounded Support Data
Source: arXiv:2606.11624 source file (2026-06-10)
Supplement: Supplementary file 5 [file cor_K.tex]

\restatealiasOn
\noindent\textbf{\Cref{cor:K}} (\corKTitle). {\itshape\corKBody}
\restatealiasOff

\begin{proof}
By~\Cref{thm:triple}, the marginal of $Y$ over $(C,A,B)$ is $\TNB(p,\,q,\,\varepsilon)$. Marginalizing only $(A,\,B)$ for fixed $C\teq c$ is the construction in~\Cref{cor:lnb_nb} with $\varepsilon$ replaced by $\varepsilon + c$, giving $Y \mid C \teq c \sim \mathrm{LNbeta}\big(\varepsilon+c,\,\varepsilon+c,\,\tfrac{1-p}{p}\big)$.
\end{proof}
\newpage
