# Supplementary material for: The Triply-Randomized Negative Binomial Beta for Robust Regression and Conjugate Models of Bounded Support Data
Source: arXiv:2606.11624 source file (2026-06-10)
Supplement: Supplementary file 6 [file cor_lnb_nb.tex]

\restatealiasOn
\noindent\textbf{\Cref{cor:lnb_nb}} (\corLnbNbTitle). {\itshape\corLnbNbBody}
\restatealiasOff
\begin{proof}
    The result follows directly from~\Cref{lemma:general_lnb} with specific parameter values.
\end{proof}
