# Supplementary material for: The Triply-Randomized Negative Binomial Beta for Robust Regression and Conjugate Models of Bounded Support Data
Source: arXiv:2606.11624 source file (2026-06-10)
Supplement: Supplementary file 7 [file prop_Kconditional.tex]

\restatealiasOn
\noindent\textbf{\Cref{prop:Kconditional}} (\propKconditionalTitle). {\itshape\propKconditionalBody}
\restatealiasOff
\begin{proof}
By~\Cref{cor:K}, $Y \mid C \teq c \sim \mathrm{LNbeta}\big(\varepsilon+c,\,\varepsilon+c,\,\tfrac{1-p}{p}\big)$ and $C \sim \mathrm{NB}(\varepsilon,\,1\tm q)$. By Bayes' rule,
\begin{align*}
    P(C \teq c \mid Y \teq y) &\propto \mathrm{LNbeta}\Big(y;\; \varepsilon \tp c,\,\varepsilon\tp c,\,\tfrac{1-p}{p}\Big)\cdot \mathrm{NB}\big(c\; \varepsilon,\, 1\tm q\big)\\
     &\propto \frac{1}{B(\varepsilon\tp c,\,\varepsilon\tp c)}\cdot\frac{\big(y(1\tm y)p(1\tm p)\big)^c}{\big(p(1\tm y) + (1\tm p)y\big)^{2c}}\cdot\frac{\Gamma(\varepsilon\tp c)}{c!}\,q^c\\
     &\propto \frac{\Gamma(2\varepsilon+2c)}{\Gamma(\varepsilon+c)}\cdot\frac{\big(\gamma(y,p) q\big)^c}{c!}
\end{align*}
where we recognize the similarity function $\gamma(y,p) = \nicefrac{y(1\tm y)p(1\tm p)}{\big(p(1\tm y) + (1\tm p)y\big)^2}$ Applying the Legendre duplication formula
$\Gamma(2z) = 2^{2z-1}\pi^{-1/2}\,\Gamma(z)\,\Gamma(z\tp\tfrac{1}{2})$ with $z = \varepsilon \tp c$ gives
\begin{equation*}
    P(C \teq c \mid Y \teq y) \propto \frac{\Gamma(\varepsilon + \tfrac{1}{2} + c)}{c!}\,\big(4q\gamma(y,p)\big)^c
\end{equation*}
which is the kernel of $\mathrm{NB}\big(\varepsilon + \tfrac{1}{2},\,1 \tm 4q\gamma(y,p)\big)$.
\end{proof}
