# Supplementary material for: The Triply-Randomized Negative Binomial Beta for Robust Regression and Conjugate Models of Bounded Support Data
Source: arXiv:2606.11624 source file (2026-06-10)
Supplement: Supplementary file 8 [file prop_con.tex]

\restatealiasOn
\noindent\textbf{\Cref{prop:con}} (\propConTitle). {\itshape\propConBody}
\restatealiasOff
\begin{proof}
We begin with the second statement and keep only terms proportional to $a$ to write
\begin{align*}
    P\big(A \teq a \mid B \teq b,\, Y \teq y\big) &\propto \mathrm{beta}\big(y;\; \varepsilon + a,\, \varepsilon + b\big)\cdot\mathrm{NB}\big(a;\,\varepsilon,\,1- p\big)\\
    &\propto \frac{\Gamma(2\varepsilon + b + a)}{a!}\big(yp\big)^{a}
\end{align*}
which is the kernel of $\mathrm{NB}\big(2\varepsilon + b,\, 1-yp\big)$.

For the first statement, we write the joint posterior over both counts. By Bayes' rule,
\begin{align*}
    P(A \teq a,\,B \teq b \mid Y \teq y) 
    &\propto \mathrm{beta}\big(y;\,\varepsilon\tp a,\,\varepsilon\tp b\big)\cdot\mathrm{NB}\big(a;\,\varepsilon,\,1\tm p\big)\cdot\mathrm{NB}\big(b;\,\varepsilon,\,p\big)\\
    &\propto \frac{\Gamma(2\varepsilon + a + b)}{a!\,b!}\,\big(yp\big)^{a}\,\big((1\tm y)(1\tm p)\big)^{b}
\end{align*}
Then marginalize over $B$ to form the posterior marginal of $A$ as
\begin{equation*}
    P(A \teq a \mid Y \teq y) \propto \frac{\big(yp\big)^{a}}{a!}\sum_{b=0}^\infty\frac{\Gamma(2\varepsilon + a + b)}{ b!}\big((1-y)(1-p)\big)^{b}.
\end{equation*}
Finally, we use the series identity $\sum_{j=0}^\infty \frac{\Gamma(\alpha+j)}{j!}x^j = \Gamma(\alpha)(1-x)^{-\alpha}$ to write
\begin{align*}
    P(A \teq a \mid Y \teq y) &\propto \frac{\Gamma(2\varepsilon + a)}{a!}\cdot\frac{\big(yp\big)^{a}}{\big(1-(1-y)(1-p)\big)^{2\varepsilon+a}}\\
    &\propto \frac{\Gamma(2\varepsilon + a)}{a!}\left(\frac{yp}{1-(1-y)(1-p)}\right)^{a}
\end{align*}
which is the kernel of $\mathrm{NB}\!\left(2\varepsilon,\,1 \tm \frac{yp}{1-(1-y)(1-p)}\right)$.
\end{proof}
