# Supplementary material for: The Triply-Randomized Negative Binomial Beta for Robust Regression and Conjugate Models of Bounded Support Data
Source: arXiv:2606.11624 source file (2026-06-10)
Supplement: Supplementary file 9 [file prop_consum.tex]

\restatealiasOn
\noindent\textbf{\Cref{prop:consum}} (\propConsumTitle). {\itshape\propConsumBody}
\restatealiasOff
\begin{proof}
For the first statement, begin from the joint inverse distribution
\begin{equation*}
    P(A \teq a,\,B \teq b \mid Y \teq y) \propto \frac{\Gamma(2\varepsilon + a + b)}{a!\,b!}\,\big(yp\big)^{a}\,\big((1\tm y)(1\tm p)\big)^{b}.
\end{equation*}
Substituting $b = s \tm a$ and summing over $a = 0,\ldots,s$:
\begin{align*}
    P\big(A + B \teq s \mid Y \teq y\big) &\propto \sum_{a=0}^{s}
     \frac{\Gamma(2\varepsilon + s)}{a!(s-a)!}\,\big(yp\big)^{a}\big((1\tm y)(1\tm p)\big)^{s-a}\\
     &\propto \frac{\Gamma(2\varepsilon + s)}{s!}
    \sum_{a=0}^{s}\binom{s}{a}\big(yp\big)^{a}\big((1\tm y)(1\tm p)\big)^{s-a}.
\end{align*}
where we used $\binom{s}{a} = s!/[a!(s\tm a)!]$. Applying the binomial theorem gives
\begin{equation*}
    P\big(A + B \teq s \mid Y \teq y\big) \propto \frac{\Gamma(2\varepsilon + s)}{s!}
    \big(yp + (1-y)(1-p)\big)^{s}
\end{equation*}
which is the kernel of $\mathrm{NB}\big(2\varepsilon,\, p(1-y) + y(1-p)\big)$.

For the second statement, we write the conditional as a ratio of the joint and marginal:
\begin{equation*}
    P\big(A \teq a \mid A + B \teq s,\,Y \teq y\big) = \frac{P(A \teq a,\,B \teq s \tm a \mid Y \teq y)}{P(A + B \teq s \mid Y \teq y)}.
\end{equation*}
Substituting the expressions above and cancelling the common factor $\Gamma(2\varepsilon+s)$:
\begin{equation*}
    P\big(A \teq a \mid A + B \teq s,\,Y \teq y\big) \propto \binom{s}{a}\big(yp\big)^{a}\big((1-y)(1-p)\big)^{s-a}
\end{equation*}
which is the kernel of $\mathrm{binomial}\!\left(s,\,\nicefrac{py}{py+(1-p)(1-y)}\right)$.
\end{proof}
