# Supplementary material for: The Triply-Randomized Negative Binomial Beta for Robust Regression and Conjugate Models of Bounded Support Data
Source: arXiv:2606.11624 source file (2026-06-10)
Supplement: Supplementary file 10 [file prop_gen.tex]

\restatealiasOn
\noindent\textbf{\Cref{prop:gen}} (\propGenTitle). {\itshape\propGenBody}
\restatealiasOff
\begin{proof}
Since $D = A + C$ and $E = B + C$, and $A$ and $B$ are independent given $C$, we marginalize $C$ noting that $D \teq d$ and $E \teq e$ constrain $C \leq d \wedge e$:
\begin{equation*}
    P(D \teq d,\, E \teq e) = \sum_{c=0}^{d \wedge e} P(A \teq d \tm c \mid C \teq c)\,P(B \teq e \tm c \mid C \teq c)\,P(C \teq c).
\end{equation*}
Expanding each negative binomial PMF in Gamma function form:
\begin{align*}
    P(A \teq d \tm c \mid C \teq c) &= \frac{\Gamma(\varepsilon + d)}{\Gamma(\varepsilon+c)\,(d - c)!}\,(1\tm p)^{\varepsilon+c}\,p^{d-c},\\
    P(B \teq e \tm c \mid C \teq c) &= \frac{\Gamma(\varepsilon + e)}{\Gamma(\varepsilon+c)\,(e - c)!}\,p^{\varepsilon+c}\,(1\tm p)^{e-c},\\
    P(C \teq c) &= \frac{\Gamma(\varepsilon + c)}{\Gamma(\varepsilon)\,c!}\,(1\tm q)^\varepsilon\,q^c.
\end{align*}
The $p$ and $(1\tm p)$ terms combine as $(1\tm p)^{\varepsilon+c}\cdot p^{d-c}\cdot p^{\varepsilon+c}\cdot(1\tm p)^{e-c} = p^{\varepsilon+d}(1\tm p)^{\varepsilon+e}$, which is independent of $c$. One factor of $\Gamma(\varepsilon + c)$ cancels between the numerator of $P(C\teq c)$ and the denominator of $P(A \teq d\tm c \mid C\teq c)$. Factoring out all terms independent of $c$:
\begin{align*}
    P(D \teq d,\,E \teq e) &= \frac{\Gamma(\varepsilon+d)\,\Gamma(\varepsilon+e)}{\Gamma(\varepsilon)}\,p^{\varepsilon+d}(1\tm p)^{\varepsilon+e}(1\tm q)^\varepsilon\sum_{c=0}^{d \wedge e}\frac{q^c}{(d-c)!\,(e-c)!\,\Gamma(\varepsilon+c)\,c!}.
\end{align*}
To evaluate the sum, we use the Pochhammer identity $1/(m\tm c)! = (-1)^c(-m)_c/m!$ so
\begin{equation*}
    \frac{1}{(d\tm c)!\,(e\tm c)!\,\Gamma(\varepsilon+c)\,c!} = \frac{(-d)_c\,(-e)_c}{d!\,e!\,\Gamma(\varepsilon)\,(\varepsilon)_c\,c!}
\end{equation*}
where $(-1)^{2c} = 1$. Last, recognize the Gauss hypergeometric series and the negative binomial mass functions $\tbinom{\varepsilon+d-1}{d}(1\tm p)^\varepsilon p^{d} = \mathrm{NB}(d;\,\varepsilon,\,1\tm p)$ and $\tbinom{\varepsilon+e-1}{e}p^\varepsilon(1\tm p)^{e} = \mathrm{NB}(e;\,\varepsilon,\,p)$ so
\begin{equation*}
    P(D \teq d,\,E \teq e) = \mathrm{NB}(d;\,\varepsilon,\,1\tm p)\cdot\mathrm{NB}(e;\,\varepsilon,\,p)\cdot(1\tm q)^\varepsilon\;{}_2F_1(-d,\,-e;\,\varepsilon;\,q). \qedhere
\end{equation*}
\end{proof}
