# Supplementary material for: The Triply-Randomized Negative Binomial Beta for Robust Regression and Conjugate Models of Bounded Support Data
Source: arXiv:2606.11624 source file (2026-06-10)
Supplement: Supplementary file 11 [file thm_triple.tex]

\begin{lemma}[\textbf{General NB-beta marginalization}]\label{lemma:general_lnb}
Let $\alpha_1,\,\alpha_2 > 0$ and $p_1,\,p_2 \in (0,1)$. Define the following auxiliary-variable randomization of a standard beta random variable
\begin{equation*}
\begin{aligned}
&J_1 \sim \mathrm{NB}(\alpha_1,\,p_1), \qquad J_2 \sim \mathrm{NB}(\alpha_2,\,p_2),\\
&Y \mid J_1 \teq j_1,\, J_2 \teq j_2 \sim \mathrm{beta}\big(\alpha_1 \tp j_1,\,\alpha_2 \tp j_2\big).
\end{aligned}
\end{equation*}
Then the marginal distribution is $Y \sim \mathrm{LNbeta}\big(\alpha_1,\,\alpha_2,\, \nicefrac{p_1}{p_2}\big)$.
\end{lemma}
\begin{proof}
We jointly marginalize $J_1$ and $J_2$. Expanding the beta and negative binomial densities and cancelling $\Gamma(\alpha_i + j_i)$ terms:
\begin{equation*}
    f(y) = \frac{y^{\alpha_1 - 1}(1-y)^{\alpha_2-1}}{B(\alpha_1,\alpha_2)}\,p_1^{\alpha_1}p_2^{\alpha_2}\sum_{j_1=0}^\infty \sum_{j_2=0}^\infty \frac{\Gamma(\alpha_1+\alpha_2+j_1+j_2)}{\Gamma(\alpha_1 +\alpha_2)\,j_1!\,j_2!}\big(y(1-p_1)\big)^{j_1}\big((1-y)(1-p_2)\big)^{j_2}.
\end{equation*}
Re-indexing with $s = j_1 + j_2$ and applying the binomial theorem to the inner sum:
\begin{align*}
    &\sum_{s=0}^\infty \frac{\Gamma(\alpha_1+\alpha_2+s)}{\Gamma(\alpha_1 +\alpha_2)\,s!}\sum_{j_1=0}^s \binom{s}{j_1}\big(y(1-p_1)\big)^{j_1}\big((1-y)(1-p_2)\big)^{s-j_1}\\
    &\qquad= \sum_{s=0}^\infty \frac{\Gamma(\alpha_1+\alpha_2+s)}{\Gamma(\alpha_1 +\alpha_2)\,s!}\big(y(1-p_1) + (1-y)(1-p_2)\big)^s.
\end{align*}
Closing the series with the identity $\sum_{s=0}^\infty \frac{\Gamma(a+s)}{\Gamma(a)\,s!}x^s = (1-x)^{-a}$ and simplifying:
\begin{equation*}
    f(y) = \frac{y^{\alpha_1-1}(1-y)^{\alpha_2-1}}{B(\alpha_1,\alpha_2)}\frac{p_1^{\alpha_1}p_2^{\alpha_2}}{\big(p_2 - (p_2-p_1)y\big)^{\alpha_1+\alpha_2}} = \frac{y^{\alpha_1-1}(1-y)^{\alpha_2-1}}{B(\alpha_1,\alpha_2)}\frac{c^{\alpha_1}}{\big(1 - (1 - c)y\big)^{\alpha_1+\alpha_2}}
\end{equation*}
where $c=\nicefrac{p_1}{p_2}$. This is the Libby-Novick beta density $\mathrm{LNbeta}(\alpha_1,\,\alpha_2,\,c)$, as in~\Cref{def:lnb}.
\end{proof}

\newpage

\restatealiasOn
\noindent\textbf{\Cref{thm:triple}} (\thmTripleTitle). {\itshape\thmTripleBody}
\restatealiasOff
\begin{proof}
By~\Cref{lemma:general_lnb} with $\alpha_1 = \alpha_2 = \varepsilon + c$, $p_1 = 1\tm p$, and $p_2 = p$, marginalizing $(A,\,B)$ for fixed $C\teq c$ gives $Y \mid C \teq c \sim \mathrm{LNbeta}\big(\varepsilon + c,\,\varepsilon + c,\,\tfrac{1-p}{p}\big)$ with density
\begin{equation*}
    f(y \mid c) = \frac{y^{\varepsilon+c-1}(1-y)^{\varepsilon+c-1}}{B(\varepsilon+c,\,\varepsilon+c)}\cdot\frac{p^{\varepsilon+c}(1\tm p)^{\varepsilon+c}}{D^{2(\varepsilon+c)}}
\end{equation*}
where $D = p(1\tm y) + (1\tm p)y$. Marginalizing $C \sim \mathrm{NB}(\varepsilon,\,1\tm q)$:
\begin{align*}
    f(y) &= \sum_{c=0}^\infty \mathrm{LNbeta}\big(y;\, \varepsilon \tp c,\,\varepsilon \tp c,\,\tfrac{1-p}{p}\big)\,\frac{\Gamma(\varepsilon + c)}{\Gamma(\varepsilon)\,c!}(1\tm q)^\varepsilon q^c\\
    &= \frac{y^{\varepsilon-1}(1-y)^{\varepsilon-1}\,p^\varepsilon(1\tm p)^\varepsilon}{D^{2\varepsilon}}\cdot(1\tm q)^\varepsilon\sum_{c=0}^\infty \frac{\Gamma(\varepsilon+c)}{\Gamma(\varepsilon)\,c!}\cdot\frac{\Gamma(2\varepsilon+2c)}{\Gamma(\varepsilon+c)^2}\cdot\left(\frac{y(1\tm y)p(1\tm p)}{D^2}\,q\right)^c
\end{align*}
where we have factored out terms independent of $c$. We simplify $\Gamma(2\varepsilon+2c)/\Gamma(\varepsilon+c)$ via the Legendre duplication formula $\Gamma(2z) = 2^{2z-1}\pi^{-1/2}\,\Gamma(z)\,\Gamma(z+\tfrac{1}{2})$:
\begin{equation*}
    \frac{\Gamma(2\varepsilon+2c)}{\Gamma(\varepsilon+c)} = \frac{2^{2\varepsilon+2c-1}}{\sqrt{\pi}}\,\Gamma\!\left(\varepsilon + c + \tfrac{1}{2}\right).
\end{equation*}
Substituting and writing $\gamma(y,p) = \nicefrac{y(1\tm y)p(1\tm p)}{D^2}$:
\begin{align*}
    f(y) &= \frac{y^{\varepsilon-1}(1-y)^{\varepsilon-1}\,p^\varepsilon(1\tm p)^\varepsilon}{D^{2\varepsilon}}\cdot(1\tm q)^\varepsilon\cdot\frac{2^{2\varepsilon-1}}{\sqrt{\pi}\,\Gamma(\varepsilon)}\sum_{c=0}^\infty \frac{\Gamma(\varepsilon+c+\tfrac{1}{2})}{c!}\,\big(4q\gamma(y,p)\big)^c.
\end{align*}
The series is $\sum_{c=0}^\infty \frac{\Gamma(\varepsilon+\frac{1}{2}+c)}{c!}(4q\gamma)^c = \Gamma\!\left(\varepsilon + \tfrac{1}{2}\right)\big(1 - 4q\gamma(y,p)\big)^{-(\varepsilon+1/2)}$. Therefore
\begin{equation*}
    f(y) = \frac{y^{\varepsilon-1}(1-y)^{\varepsilon-1}\,p^\varepsilon(1\tm p)^\varepsilon}{D^{2\varepsilon}}\cdot(1\tm q)^\varepsilon\cdot\frac{2^{2\varepsilon-1}\,\Gamma(\varepsilon+\tfrac{1}{2})}{\sqrt{\pi}\,\Gamma(\varepsilon)}\cdot(1 - 4q\gamma)^{-(\varepsilon+1/2)}.
\end{equation*}
Applying the duplication formula once more gives $\frac{2^{2\varepsilon-1}\,\Gamma(\varepsilon+\frac{1}{2})}{\sqrt{\pi}\,\Gamma(\varepsilon)} = \frac{\Gamma(2\varepsilon)}{\Gamma(\varepsilon)^2} = \frac{1}{B(\varepsilon,\varepsilon)}$, so
\begin{equation*}
    f(y) = \frac{y^{\varepsilon-1}(1-y)^{\varepsilon-1}}{B(\varepsilon,\varepsilon)}\cdot\frac{p^\varepsilon(1\tm p)^\varepsilon}{D^{2\varepsilon}}\cdot\frac{(1\tm q)^\varepsilon}{(1 - 4q\gamma(y,p))^{\varepsilon+1/2}} = \TNB(y;\,p,\,q,\,\varepsilon). \qedhere
\end{equation*}
\end{proof}
