# Supplementary material for: The Triply-Randomized Negative Binomial Beta for Robust Regression and Conjugate Models of Bounded Support Data
Source: arXiv:2606.11624 source file (2026-06-10)
Supplement: Supplementary file 12 [file C_experiment_details.tex]

\section{Experimental Details}\label{sec:app_exp}

We provide additional dataset and computational details for the experiments in~\Cref{sec:experiments}. For the model implementations in each experiment, we use Stan~\citep{carpenter_stan_2017} for all beta regression models and the code provided by~\cite{lee2026scalable} for cobin and micobin models. We modify the micobin code for ICAR random effects for the experiments in~\Cref{sec:trees}. To implement TNBbeta models, we use existing Pólya-gamma samplers~\citep{polson_bayesian_2013,windle_sampling_2014}.

\subsection{\Cref{sec:bench} Details}\label{sec:app_datasets}

\Cref{tab:datasets} summarizes the seven datasets used in the experiments of~\Cref{sec:bench}.
All predictors are centered and standardized prior to fitting, and an intercept column is appended.
A random 10\% holdout set is used for predictive evaluation in each model fit.

The two synthetic datasets are generated from a beta regression model with $Y_i \sim \textrm{beta}(\mu_i \phi,\, (1-\mu_i)\phi)$, $\mu_i = \textrm{logit}^{-1}(X_i^\top \beta)$, $\phi = 5$, and $\beta_j \sim \mathcal{N}(0, 0.2)$ for each coefficient including the intercept.
The orthogonal design matrix is constructed via QR decomposition of a Gaussian matrix.
The collinear design matrix is constructed from a 5-factor Gaussian factor model with additive noise.

\begin{table}[ht]
\centering
\caption{Datasets used in the~\Cref{sec:bench} experiments. $n$ is the number of observations and $p$ is the number of predictors (excluding the intercept).}
\label{tab:datasets}
\small
\begin{tabular}{llrrl}
\toprule
Dataset & Response $Y$ & $n$ & $p$ & Source \\
\midrule
AlcoholUse & Alcohol use percentage & 1{,}340 & 3 & \texttt{zoib} R package \\
Bike & Casual / total rentals & 731 & 11 & UCI ML Repository (ID 275) \\
Credit & Recent payment ratio & 18{,}150 & 11 & UCI ML Repository (ID 350) \\
Crime & Violent crimes per capita & 1{,}940 & 20 & UCI ML Repository (ID 183) \\
Productivity & Actual productivity & 1{,}160 & 10 & UCI ML Repository (ID 597) \\
Synthetic (orth.) & Simulated beta & 500 & 20 & Generated \\
Synthetic (corr.) & Simulated beta & 500 & 20 & Generated \\
\bottomrule
\end{tabular}
\end{table}

\Cref{tab:ess_single} reports the effective sample size and wall-clock time for each model in the shared concentration experiment. Furthermore,~\Cref{tab:bench_dispreg} reports the information rate, effective sample size, ESS per second, and wall-clock time for the concentration regression experiment. Last,~\Cref{tab:bench_nostd} shows the results in the shared concentration setting on data without covariate standardization, which can have a large negative effect on the computational efficiency of beta regression via HMC while the results for the TNBbeta are largely unchanged.

\begin{table}[ht]
\centering
\caption{ESS and wall-clock time (seconds) for shared concentration models.}
\label{tab:ess_single}
% Auto-generated by export_results.R
% Do not edit manually.

\small
\begin{tabular}{l cc cc cc cc}
\toprule
  & \multicolumn{2}{c}{TNBbeta} & \multicolumn{2}{c}{Beta} & \multicolumn{2}{c}{Cobin} & \multicolumn{2}{c}{Micobin} \\
 \cmidrule(lr){2-3} \cmidrule(lr){4-5} \cmidrule(lr){6-7} \cmidrule(lr){8-9}
Dataset & ESS & Time (s) & ESS & Time (s) & ESS & Time (s) & ESS & Time (s) \\
\midrule
Orthogonal & 905 \scriptsize{(4)} & 2.5 & 4655 \scriptsize{(66)} & 3.7 & 1389 \scriptsize{(10)} & 6.5 & 1003 \scriptsize{(4)} & 15.0 \\
Collinear & 945 \scriptsize{(5)} & 2.7 & 2981 \scriptsize{(71)} & 17.1 & 1679 \scriptsize{(11)} & 6.5 & 1169 \scriptsize{(6)} & 15.8 \\
Bike & 677 \scriptsize{(4)} & 2.5 & 1764 \scriptsize{(28)} & 27.5 & 763 \scriptsize{(7)} & 18.5 & 483 \scriptsize{(4)} & 40.5 \\
Product & 952 \scriptsize{(6)} & 6.0 & 2703 \scriptsize{(34)} & 11.4 & 1221 \scriptsize{(10)} & 13.2 & 775 \scriptsize{(9)} & 41.6 \\
Alcohol & 681 \scriptsize{(11)} & 6.8 & 1811 \scriptsize{(19)} & 6.1 & 173 \scriptsize{(4)} & 18.0 & 168 \scriptsize{(2)} & 46.8 \\
Crime & 851 \scriptsize{(4)} & 11.0 & 1789 \scriptsize{(19)} & 127.5 & 1056 \scriptsize{(6)} & 21.6 & 737 \scriptsize{(4)} & 58.4 \\
Credit & 954 \scriptsize{(5)} & 93.4 & 2595 \scriptsize{(39)} & 138.2 & 428 \scriptsize{(2)} & 113.8 & 420 \scriptsize{(2)} & 404.1 \\
\bottomrule
\end{tabular}

\end{table}

\begin{table}[ht]
\centering
\caption{TNBbeta regression models with covariates on the concentration parameter tend to match or improve on prediction and efficiency of the analogous beta models.}
\label{tab:bench_dispreg}
% Auto-generated by export_results.R
% Do not edit manually.

\small
\setlength{\tabcolsep}{3pt}
\begin{tabular}{l cc cccc cccc}
\toprule
 & &  & \multicolumn{4}{c}{TNBbeta} & \multicolumn{4}{c}{Beta} \\
 \cmidrule(lr){4-7} \cmidrule(lr){8-11}
Dataset & $n$ & $p$ & IR $(\downarrow)$ & ESS & sec & $\nicefrac{\textrm{ESS}}{\textrm{sec}}$ & IR $(\downarrow)$ & ESS & sec & $\nicefrac{\textrm{ESS}}{\textrm{sec}}$ \\
\midrule
Orthogonal & 500 & 20 & -0.31 \scriptsize{(0.02)} & 495 \scriptsize{(9)} & 3.3 & 149 & \textbf{-0.41 \scriptsize{(0.02)}} & 2407 \scriptsize{(39)} & 5.2 & \textbf{462} \\[2pt]
Collinear & 500 & 20 & \textbf{-0.29 \scriptsize{(0.02)}} & 715 \scriptsize{(4)} & 4.1 & \textbf{174} & \textbf{-0.31 \scriptsize{(0.02)}} & 3380 \scriptsize{(47)} & 25.5 & 133 \\[2pt]
Bike & 731 & 11 & \textbf{-1.65 \scriptsize{(0.02)}} & 586 \scriptsize{(6)} & 5.4 & \textbf{109} & \textbf{-1.64 \scriptsize{(0.03)}} & 1945 \scriptsize{(52)} & 30.6 & 64 \\[2pt]
Product & 1,160 & 10 & \textbf{-0.94 \scriptsize{(0.02)}} & 770 \scriptsize{(16)} & 7.5 & \textbf{103} & -0.65 \scriptsize{(0.03)} & 1698 \scriptsize{(36)} & 21.4 & 79 \\[2pt]
Alcohol & 1,288 & 3 & -2.26 \scriptsize{(0.02)} & 496 \scriptsize{(10)} & 10.4 & 48 & \textbf{-2.31 \scriptsize{(0.02)}} & 2111 \scriptsize{(37)} & 7.5 & \textbf{281} \\[2pt]
Crime & 1,940 & 20 & \textbf{-1.00 \scriptsize{(0.02)}} & 769 \scriptsize{(6)} & 19.1 & \textbf{40} & \textbf{-0.97 \scriptsize{(0.02)}} & 2010 \scriptsize{(27)} & 187.9 & 11 \\[2pt]
Credit & 18,150 & 11 & \textbf{-1.35 \scriptsize{(0.01)}} & 656 \scriptsize{(5)} & 152.6 & 4 & -1.03 \scriptsize{(0.01)} & 2331 \scriptsize{(30)} & 295.3 & \textbf{8} \\
\bottomrule
\end{tabular}

\end{table}

\begin{table}
\centering
\caption{Shared concentration results without covariate standardization. HMC efficiency is sensitive to the magnitude of the covariates.}
\label{tab:bench_nostd}
% Auto-generated by export_results.R
% Do not edit manually.

\small
\setlength{\tabcolsep}{3pt}
\begin{tabular}{l cc cc cc cc cc}
\toprule
 & &  & \multicolumn{2}{c}{TNBbeta} & \multicolumn{2}{c}{Beta} & \multicolumn{2}{c}{Cobin} & \multicolumn{2}{c}{Micobin} \\
 \cmidrule(lr){4-5} \cmidrule(lr){6-7} \cmidrule(lr){8-9} \cmidrule(lr){10-11}
Dataset & $n$ & $p$ & IR $(\downarrow)$ & $\nicefrac{\textrm{ESS}}{\textrm{sec}}$ & IR $(\downarrow)$ & $\nicefrac{\textrm{ESS}}{\textrm{sec}}$ & IR $(\downarrow)$ & $\nicefrac{\textrm{ESS}}{\textrm{sec}}$ & IR $(\downarrow)$ & $\nicefrac{\textrm{ESS}}{\textrm{sec}}$ \\
\midrule
Orthogonal & 500 & 20 & -0.35 \scriptsize{(0.02)} & 368 & \textbf{-0.42 \scriptsize{(0.02)}} & \textbf{1105} & -0.32 \scriptsize{(0.03)} & 211 & -0.35 \scriptsize{(0.02)} & 64 \\[2pt]
Collinear & 500 & 20 & \textbf{-0.31 \scriptsize{(0.02)}} & \textbf{352} & \textbf{-0.33 \scriptsize{(0.02)}} & 169 & \textbf{-0.31 \scriptsize{(0.02)}} & 253 & \textbf{-0.31 \scriptsize{(0.02)}} & 72 \\[2pt]
Bike & 731 & 11 & \textbf{-1.60 \scriptsize{(0.02)}} & \textbf{289} & \textbf{-1.58 \scriptsize{(0.02)}} & 36 & -1.45 \scriptsize{(0.02)} & 57 & -1.48 \scriptsize{(0.02)} & 18 \\[2pt]
Product & 1,160 & 10 & \textbf{-0.67 \scriptsize{(0.01)}} & \textbf{161} & -0.56 \scriptsize{(0.01)} & $<$1 & -0.54 \scriptsize{(0.01)} & 99 & -0.61 \scriptsize{(0.02)} & 19 \\[2pt]
Alcohol & 1,288 & 3 & -2.18 \scriptsize{(0.02)} & \textbf{103} & \textbf{-2.30 \scriptsize{(0.02)}} & 99 & \textbf{-2.31 \scriptsize{(0.02)}} & 13 & \textbf{-2.31 \scriptsize{(0.01)}} & 4 \\[2pt]
Crime & 1,940 & 20 & \textbf{-0.99 \scriptsize{(0.02)}} & \textbf{98} & -0.88 \scriptsize{(0.02)} & 7 & -0.92 \scriptsize{(0.02)} & 70 & -0.90 \scriptsize{(0.02)} & 21 \\[2pt]
Credit & 18,150 & 11 & \textbf{-1.28 \scriptsize{(0.01)}} & \textbf{11} & -0.57 \scriptsize{(0.00)} & $<$1 & -1.17 \scriptsize{(0.01)} & 4 & -1.17 \scriptsize{(0.01)} & 1 \\
\bottomrule
\end{tabular}

\end{table}

\subsection{\Cref{sec:trees} Details}\label{sec:app_spatial}

\Cref{tab:covariates} describes the six environmental covariates associated with each site in the tree canopy dataset of~\Cref{sec:trees}.
All covariates are centered and standardized prior to fitting, and an intercept is appended, giving $p=7$ columns in the design matrix.

\begin{table}[ht]
\centering
\caption{Environmental covariates for the tree canopy dataset. Each covariate is computed as the average within the corresponding $20 \!\times\! 20$ meter cell.}
\label{tab:covariates}
\small
\begin{tabular}{ll}
\toprule
Covariate & Description \\
\midrule
\texttt{wetness} & Topographic wetness index \\
\texttt{southness} & Aspect southness component \\
\texttt{degreedays} & Growing degree days \\
\texttt{dem} & Digital elevation (meters) \\
\texttt{slope} & Slope steepness (degrees) \\
\texttt{snowpack} & Snowpack persistence \\
\bottomrule
\end{tabular}
\end{table}

The dataset consists of a $100 \!\times\! 100$ grid of cells covering the Upper Gunnison Watershed, yielding $10{,}000$ cells.
For the beta regression comparison, we discard all sites with exactly $0\%$ canopy, leaving $N = 8{,}763$ observations as described in~\Cref{sec:trees}.
The spatial adjacency matrix uses 4-neighbor connectivity.

For the $K$-fold cross-validation experiments, we use $K = 20$ folds defined by deterministic $10 \!\times\! 10$ spatial blocks.
Each fold is fit with $4$ chains, $2{,}000$ burn-in iterations, and $1{,}000$ sampling iterations.
For the full-data fits used in~\Cref{fig:canopy}, we use $4$ chains with $5{,}000$ burn-in and $2{,}000$ sampling iterations, fit to all $10,\!000$ sites.
\Cref{tab:tree_timing} reports the MCMC sampling time and information rate computation time for each model, averaged over the $20$ cross-validation replications on identical hardware.

\begin{table}[ht]
\centering
\caption{MCMC sampling time and held-out information rate computation time for each tree canopy model, averaged over folds, in seconds.}
\label{tab:tree_timing}
% Auto-generated by export_results.R
% Do not edit manually.

\small
\setlength{\tabcolsep}{4pt}
\begin{tabular}{l cc cc cc}
\toprule
 & \multicolumn{2}{c}{TNBbeta} & \multicolumn{2}{c}{Beta (HMC)} & \multicolumn{2}{c}{Micobin} \\
\cmidrule(lr){2-3} \cmidrule(lr){4-5} \cmidrule(lr){6-7}
Model & MCMC & IR & MCMC & IR & MCMC & IR \\
\midrule
Cov + Scalar & 70 \scriptsize{(1)} & 31 \scriptsize{(2)} & 544 \scriptsize{(3)} & 12 \scriptsize{(1)} & 142 \scriptsize{(2)} & 858 \scriptsize{(29)} \\
Cov + Cov & 64 \scriptsize{(1)} & 25 \scriptsize{(2)} & 464 \scriptsize{(16)} & 16 \scriptsize{(1)} & 194 \scriptsize{(2)} & 840 \scriptsize{(33)} \\
ICAR + Scalar & 89 \scriptsize{(2)} & 17 \scriptsize{(2)} & 2009 \scriptsize{(47)} & 11 \scriptsize{(1)} & 704 \scriptsize{(19)} & 796 \scriptsize{(30)} \\
ICAR + Cov & 95 \scriptsize{(2)} & 15 \scriptsize{(2)} & 3486 \scriptsize{(170)} & 11 \scriptsize{(1)} & 664 \scriptsize{(22)} & 719 \scriptsize{(24)} \\
\bottomrule
\end{tabular}

\end{table}
