# Supplementary material for: The Triply-Randomized Negative Binomial Beta for Robust Regression and Conjugate Models of Bounded Support Data
Source: arXiv:2606.11624 source file (2026-06-10)
Supplement: Supplementary file 13 [file benchmark_appendix_table.tex]

% Auto-generated by export_results.R
% Do not edit manually.

\small
\begin{tabular}{l cc cc cc cc}
\toprule
  & \multicolumn{2}{c}{TNBbeta} & \multicolumn{2}{c}{Beta} & \multicolumn{2}{c}{Cobin} & \multicolumn{2}{c}{Micobin} \\
 \cmidrule(lr){2-3} \cmidrule(lr){4-5} \cmidrule(lr){6-7} \cmidrule(lr){8-9}
Dataset & ESS & Time (s) & ESS & Time (s) & ESS & Time (s) & ESS & Time (s) \\
\midrule
Orthogonal & 905 \scriptsize{(4)} & 2.5 & 4655 \scriptsize{(66)} & 3.7 & 1389 \scriptsize{(10)} & 6.5 & 1003 \scriptsize{(4)} & 15.0 \\
Collinear & 945 \scriptsize{(5)} & 2.7 & 2981 \scriptsize{(71)} & 17.1 & 1679 \scriptsize{(11)} & 6.5 & 1169 \scriptsize{(6)} & 15.8 \\
Bike & 677 \scriptsize{(4)} & 2.5 & 1764 \scriptsize{(28)} & 27.5 & 763 \scriptsize{(7)} & 18.5 & 483 \scriptsize{(4)} & 40.5 \\
Product & 952 \scriptsize{(6)} & 6.0 & 2703 \scriptsize{(34)} & 11.4 & 1221 \scriptsize{(10)} & 13.2 & 775 \scriptsize{(9)} & 41.6 \\
Alcohol & 681 \scriptsize{(11)} & 6.8 & 1811 \scriptsize{(19)} & 6.1 & 173 \scriptsize{(4)} & 18.0 & 168 \scriptsize{(2)} & 46.8 \\
Crime & 851 \scriptsize{(4)} & 11.0 & 1789 \scriptsize{(19)} & 127.5 & 1056 \scriptsize{(6)} & 21.6 & 737 \scriptsize{(4)} & 58.4 \\
Credit & 954 \scriptsize{(5)} & 93.4 & 2595 \scriptsize{(39)} & 138.2 & 428 \scriptsize{(2)} & 113.8 & 420 \scriptsize{(2)} & 404.1 \\
\bottomrule
\end{tabular}
